# Supplementary material for: Automatically Labeling Clinical Trial Outcomes: A Large-Scale Benchmark for Drug Development
Source: arXiv:2406.10292 source file (2025-03-06)
Supplement: Supplementary file 1 [file supplementary.tex]

% \documentclass[11pt]{article}

% % Language setting
% % Replace `english' with e.g. `spanish' to change the document language
% \usepackage[english]{babel}
% % \usepackage{ctex}
% \usepackage{amssymb}
% \usepackage{amsmath}
% \usepackage{pdfpages}
% \usepackage{caption}
% % Set page size and margins
% % Replace `letterpaper' with `a4paper' for UK/EU standard size
% \usepackage[letterpaper,top=2cm,bottom=2cm,left=3cm,right=3cm,marginparwidth=1.75cm]{geometry}
% \usepackage{pifont}
% \newcommand{\cmark}{{\color{teal}\ding{51}}}
% \newcommand{\xmark}{{\color{red}\ding{55}}}
% % Useful packages
% \usepackage{amsmath}
% \usepackage{graphicx}
% \usepackage[colorlinks=true, linkcolor=black, citecolor=blue]{hyperref}
% % \usepackage{lineno}
% \usepackage{color}
% \usepackage{xcolor}
% \usepackage{multirow}
% \usepackage{booktabs}
% \usepackage{xspace}
% \usepackage{setspace}
% \usepackage{float}
% \usepackage{bm}

% \newcommand{\ourM}{ActFound}
% \newcommand{\ourmodel}{Panacea\xspace}

% \newcommand{\ZX}[1]{{\bf\color{red}[{ZX: #1}]}}
% \newcommand{\revise}[1]{{\color{red}{#1}}}


% \usepackage{graphicx} % For including graphics
% \usepackage{caption}  % For caption customization

% \usepackage{enumitem}
% \newcounter{suppfigure}
% \renewcommand{\thesuppfigure}{\arabic{suppfigure}} % S1, S2, S3...

% \author{Chufan Gao$^{*}$, Jathurshan Pradeepkumar$^{*}$, Trisha Das$^{*}$, Shivashankar Thati and \\ Jimeng Sun\\
% Department of Computer Science, University of Illinois Urbana-Champaign \\
% $^*$ Equal contribution \\
% Corresponding authors: \texttt{jimeng@illinois.edu}}





% % \newcommand{\suppfigurecaption}[1]{
% %   \refstepcounter{suppfigure} % 增加计数器的值
% %   \caption*{\textbf{Supplementary Figure \thesuppfigure:} #1} % 创建不带编号的标题
% % }

% \usepackage{titletoc}
% \newcommand\DoToC{%
%   \startcontents
%   \printcontents{}{1}{\textbf{Contents}\vskip3pt\hrule\vskip5pt}
%   \vskip3pt\hrule\vskip5pt
% }
% \newcommand{\mycomment}[1]{}
% \newcommand{\method}{\text{CTO}\xspace}
% \newcommand{\andy}[1]{{\small\color{red}{\bf andy:} #1}}
% \newcommand{\trisha}[1]{{\small\color{violet}{\bf Trisha:} #1}}
% \newcommand{\jathu}[1]{{\small\color{blue}{\bf Jathu:} #1}}

% \makeatletter
% \renewcommand{\maketitle}{\bgroup\setlength{\parindent}{0pt}
% \begin{flushleft}
%   \textbf{\@title}

%   \@author
% \end{flushleft}\egroup
% }
% \makeatother


% \title{Supplementary Materials: Automatically Labeling Clinical Trial Outcomes: A Large-Scale Benchmark for
% Drug Development}



% \begin{document}

% \maketitle
% % \linenumbers


% \appendix
% % \DoToC
% % \newpage



% \section*{Ethics and Broader Impacts}
% Using a weakly supervised dataset for clinical trial outcome prediction with large language models (LLMs) can potentially decrease the reliability of the model's predictions if not correctly instantiated with proper labeling functions. Weak supervision may result in incomplete or imprecise labeling, leading to the model learning incorrect associations and missing crucial factors, which can introduce or exacerbate biases. This lack of precise guidance can also cause the model to overfit to noise or incorrect patterns in the training data, reducing its ability to generalize effectively to new, unseen data. In diverse clinical scenarios, one must take care to independently verify model predictions to prevent potentially jeopardizing patient safety with inaccurate predictions. To mitigate these issues, it is essential to improve the quality of the training data through better labeling techniques, supplementary high-quality data, or advanced methods like semi-supervised or active learning.

% Furthermore, we use publicly available data, so the risk of identification is minimized. However, we recognize that LLMs on public data inherently still pose some privacy risks.

% \paragraph*{Reproducibility}
% We utilized an AMD EPYC 7513 32-core Processor with 100 GB of RAM to run our experiments. Running Data Programming with less or more powerful systems may impact speed. For us, obtaining the labels took around 25 hours in experiments and prototyping. Additionally, we made use of ChatGPT for writing as well as obtaining trial outcome prediction on the PubMed abstracts. Total cost was around \$200 US dollars.

% \section*{Related Work}



% \begin{table}[ht]
% \centering
% \caption{This table describes an overview of selected recent trial outcome prediction work. All previous work relies on industry sponsors to obtain labels, and most are not easily accessible. We are the first to aggregate publicly available data sources on a large number of trials.}
% \label{tab:prevwork}
% \Huge
% \resizebox{\linewidth}{!}{
% \begin{tabular}{llllcc} 
% \toprule[1pt]
% \textbf{Dataset} & \textbf{Data Sponsor} & \textbf{Subset} & \textbf{\# Trials} & \textbf{Label Creation} & \begin{tabular}[c]{@{}l@{}}\textbf{Publicly} \\ \textbf{Available}\end{tabular} \\ \midrule
% Lo et al. \cite{lo2019machine} & TrialTrove, Pharmaprojects & Phase II, III & 19,136 & Human Expert & \xmark \\
% Feijoo et al. \cite{feijoo2020key} & Biomedtracker & Industry Phase II, III & 6,417 & Manual linking & \xmark \\
% % Aliper et al. \cite{aliper2023prediction} & Insilico Medicine & Phase II & 55,653 & Biomedical KG, Trial stats & \xmark \\
% Aliper et al. \cite{aliper2023prediction} & Insilico Medicine & Phase II & 55,653 & Human Expert & \xmark \\
% Willigers et al. \cite{willigers2023algorithmic} & AstraZeneca & AstraZeneca Phase III & 57 & Human Expert & \xmark \\
% TOP \cite{fu2022hint} & IQVIA & Small Molecule Drugs & 17,538 & Human Expert & \cmark \\ \midrule
% \method\ (ours) & Publicly Collected & All & 125,840 & \begin{tabular}[c]{@{}l@{}}Automatic Aggregation \\ (Tuned by Human Labeling)\end{tabular} & \cmark \\ \bottomrule[0.8pt]
% \end{tabular}
% }
% % \vspace{-.5em}
% \end{table}

% Predicting clinical trial outcomes is often led by industries with the capacity for extensive data curation. Informa's TrialTrove \cite{stergiopoulos2019evaluating} is widely used, containing around 20,000 trials \cite{lo2019machine}. AstraZeneca has developed structured feedback forms to improve Phase 3 trial success annotations \cite{willigers2023algorithmic}. Feijoo et al. \cite{feijoo2020key} demonstrated that using Random Forest on Biomedtracker, a proprietary dataset aggregating company reports, results in strong outcome prediction performance.

% Previous studies have tackled clinical trial outcome prediction using various methods. Early work employed statistical analysis \cite{malik2014predicting} and ML models on limited private data sets ($<$500 samples) \cite{dimasi2015tool}. In drug toxicity prediction, Gayvert et al. \cite{gayvert2016data} used Random Forest to predict outcomes based on chemical properties. In contrast, Artemov et al. \cite{artemov2016integrated} used Multi-layer Perceptrons (MLP) for Phase I/II trials. Lo et al. \cite{lo2019machine} applied k-NN imputation and Random Forest on features from Pharmaprojects and TrialTrove. Additionally, Phase 2 to Phase 3 prediction was explored by Qi et al. \cite{qi2019predicting} through clinical trials and by Aliper et al. \cite{aliper2023prediction} using experts, GPT-3.5, and a biomedical knowledge graph.

% Previous works have addressed clinical trial outcome prediction in various ways, with early work focusing on statistical analysis \cite{malik2014predicting} and ML models on small amounts of private outcome labels \cite{dimasi2015tool} (<500 samples).
% A related field is drug toxicity prediction, where Gayvert et al. \cite{gayvert2016data} used Random Forest to predict drug toxicity outcomes from chemical properties and target-based features including molecular weight and polar surface area. Similarly, Artemov et al. \cite{artemov2016integrated} used Multilayer Perceptions to predict the toxicities and outcomes of Phase I/II drugs clinical trials. 

% Lo et al. \cite{lo2019machine} used K-nearest-neighbor (KNN) imputation and Random Forest (RF) to predict outcomes on features from two commercial databases, Pharmaprojects and Trialtrove. 
% Additionally, Phase 2 to Phase 3 prediction has been explored \cite{qi2019predicting, aliper2023prediction}, However, Qi et al. \cite{qi2019predicting} conducted their clinical trial to obtain the data, and Aliper et al. \cite{aliper2023prediction} used experts, GPT3.5, as well as a proprietary biomedical knowledge graph to annotate their transition success labels for phase 2 trials. 

% Fu et al. \cite{fu2023automated} released the first \textit{and only} publicly available clinical trial outcome dataset based on manual curation. Train and test data splits were selected as all trials completed before 2014 and afterward respectively. After preprocessing and cleaning, the final number of trials in train, validation, and test datasets was reduced to 17,538 $\rightarrow$ 12,465 trials, which was only around 4\% of all available trials at the time of publication \footnote{Note that the full set of small-molecule drug interventional trials, which TOP primarily focuses on, consists of around 100k trials}. Table~\ref{tab:prevwork} summarizes recent trial outcome work.

% % \subsection*{Resources on obtaining trial data}
% % \begin{enumerate}
% %     \item Downloading all data, select pipe-delimited files. Match indexes by NCTID \url{https://aact.ctti-clinicaltrials.org/download} For consistency, we used the date \texttt{20231218\_clinical\_trials.zip}

% %     \item Downloading from the official site. Top-level data only, many details, including eligibility criteria, are missing. \url{https://clinicaltrials.gov/search}
% % \end{enumerate}


% % \section*{Previous Work}

% \section*{Benchmarking Baselines on Manually Curated Trial Outcome Benchmark}

% \begin{table}[t!]
% \centering
% \caption{Table of performance of baseline model on only the human-label subset. Training data were trials that had completion dates $<2022$ and test data were trials that had completion dates $\geq 2022$.}
% \label{tab:humanlabel}
% \resizebox{.5\linewidth}{!}{
% \begin{tabular}{cclll} \toprule
% Phase              & Model      & F1                 & PRAUC              & ROCAUC             \\ \midrule
% \multirow{7}{*}{1} & RF         & 0.790$_{\pm0.011}$ & 0.743$_{\pm0.015}$ & 0.544$_{\pm0.011}$ \\
%                    & LR         & 0.750$_{\pm0.010}$ & 0.766$_{\pm0.013}$ & 0.585$_{\pm0.015}$ \\
%                    & XGBoost    & 0.786$_{\pm0.011}$ & 0.739$_{\pm0.014}$ & 0.546$_{\pm0.012}$ \\
%                    & MLP        & 0.771$_{\pm0.010}$ & 0.748$_{\pm0.013}$ & 0.562$_{\pm0.013}$ \\
%                    & SVM        & 0.781$_{\pm0.010}$ & 0.741$_{\pm0.012}$ & 0.546$_{\pm0.012}$ \\
%                    & BioBERT    & 0.745$_{\pm0.010}$ & 0.763$_{\pm0.014}$ & 0.556$_{\pm0.015}$ \\
%                    & PubMedBERT & 0.761$_{\pm0.011}$ & 0.758$_{\pm0.015}$ & 0.546$_{\pm0.014}$ \\ \midrule
% \multirow{7}{*}{2} & RF         & 0.675$_{\pm0.009}$ & 0.652$_{\pm0.011}$ & 0.581$_{\pm0.012}$ \\
%                    & LR         & 0.646$_{\pm0.008}$ & 0.655$_{\pm0.01}$  & 0.579$_{\pm0.010}$  \\
%                    & XGBoost    & 0.696$_{\pm0.009}$ & 0.665$_{\pm0.012}$ & 0.585$_{\pm0.011}$ \\
%                    & MLP        & 0.653$_{\pm0.009}$ & 0.658$_{\pm0.012}$ & 0.567$_{\pm0.012}$ \\
%                    & SVM        & 0.683$_{\pm0.009}$ & 0.650$_{\pm0.010}$ & 0.571$_{\pm0.011}$ \\
%                    & BioBERT    & 0.659$_{\pm0.009}$ & 0.651$_{\pm0.011}$ & 0.567$_{\pm0.011}$ \\
%                    & PubMedBERT & 0.670$_{\pm0.010}$ & 0.636$_{\pm0.011}$ & 0.550$_{\pm0.011}$  \\ \midrule
% \multirow{7}{*}{3} & RF         & 0.581$_{\pm0.013}$ & 0.607$_{\pm0.011}$ & 0.606$_{\pm0.011}$ \\
%                    & LR         & 0.601$_{\pm0.015}$ & 0.603$_{\pm0.012}$ & 0.615$_{\pm0.014}$ \\
%                    & XGBoost    & 0.584$_{\pm0.012}$ & 0.594$_{\pm0.011}$ & 0.597$_{\pm0.011}$ \\
%                    & MLP        & 0.599$_{\pm0.014}$ & 0.581$_{\pm0.012}$ & 0.607$_{\pm0.014}$ \\
%                    & SVM        & 0.589$_{\pm0.013}$ & 0.587$_{\pm0.011}$ & 0.600$_{\pm0.012}$   \\
%                    & BioBERT    & 0.588$_{\pm0.012}$ & 0.560$_{\pm0.012}$ & 0.588$_{\pm0.012}$ \\
%                    & PubMedBERT & 0.601$_{\pm0.013}$ & 0.567$_{\pm0.012}$ & 0.599$_{\pm0.013}$ \\ \bottomrule
% \end{tabular}
% }
% \end{table}


% % \andy{add a table for baseline results on our gold set}

% Table~\ref{tab:humanlabel} summarizes the performance of various baseline models on our CTO gold labels, where training was conducted using our manually labeled gold set trials completed before 2022, and testing was done on trials completed post-2022. Performance metrics include F1 score, Precision-Recall Area Under the Curve (PRAUC), and Receiver Operating Characteristic Area Under the Curve (ROCAUC). Each performance measure is weighted by label prevalence to ensure a fair comparison of both positive and negative classes. 

% RF denotes random forest, LR denotes logistic regression, MLP denotes multilayer perception with 1 hidden layer of dimension 100, and SVM is the Support Vector Machine linear classifier. The input features are the term-frequency times inverse document-frequency (TFIDF) transformation of the concatenated trial phase, disease, interventions, design, and inclusion/exclusion criteria. 
% For BioBERT and PubMedBERT, we use both of these large language models (LLMs) to encode the input text (instead of TFIDF) to obtain embedding features on which a 2-layer MLP with hidden dimension 100 is trained. 

% Advanced trial outcome models, such as HINT \cite{fu2022hint} and SPOT \cite{wang2023spot}, present notable limitations that hinder their adaptability to newer clinical trials. Both approaches rely on pretrained models to predict ADMET properties—absorption, distribution, metabolism, excretion, and toxicity. However, in our evaluations, these pretrained models demonstrated suboptimal adaptability when applied to novel drugs and biologics, likely due to domain shifts or insufficient representation of emerging compounds. While optimizing these sophisticated techniques is highly valuable, our primary focus in this study is the development and curation of the dataset, laying the groundwork for better trial modeling for future work.

% In Phase 1, models demonstrated strong overall performance, with Random Forest (RF) achieving the highest F1 score (0.79), closely followed by XGBoost (0.786) and Support Vector Machines (SVM, 0.781). Logistic Regression (LR) excelled in terms of precision-recall trade-offs, reflected in its highest PRAUC (0.766) and ROCAUC (0.585) scores, suggesting superior discriminative ability in this phase. 
% Interestingly, large language models--BioBERT and PubMedBERT-- underperformed slightly in F1 scores. This could be due to the possible overfitting on the training set, as these models are much larger than the classical ones, and we see in the original paper that distribution shift is an issue over each consecutive year.

% In Phase 2, performance declined across all models, suggesting increased complexity or noise in the dataset. XGBoost emerged as the most robust model, achieving the highest F1 score (0.696), PRAUC (0.665), and ROCAUC (0.585). RF (F1: 0.675) and SVM (F1: 0.683) also showed resilience, maintaining consistent performance. However, deep learning models exhibited a pronounced decline, with PubMedBERT and BioBERT achieving lower F1 scores (0.67 and 0.659, respectively) and showing limited adaptation to the challenges of this phase. These findings emphasize the robustness of XGBoost and the potential limitations of pre-trained transformer-based models when applied to datasets with phase-specific complexities.

% Phase 3 presented the greatest challenges, with performance metrics reaching their lowest levels. Logistic Regression demonstrated the most robust performance, achieving the highest F1 score (0.601) and ROCAUC (0.615), indicative of its adaptability to the phase's complexities. PubMedBERT performed comparably in terms of F1 (0.601) but lagged in precision-recall balance, as evidenced by its lower PRAUC (0.567). Classical models such as RF and XGBoost performed moderately but did not exhibit the same dominance seen in earlier phases. Deep learning models struggled consistently across all metrics in Phase 3, suggesting that their reliance on pre-trained features may not generalize effectively to this phase's data distribution.

% Across all phases, a clear trend of declining performance from Phase 1 to Phase 3 was observed, potentially due to increasing data complexity, reduced signal strength, or distributional shifts in the features. Classical models, particularly XGBoost and RF, were robust in Phases 1 and 2, while Logistic Regression excelled in Phase 3, highlighting the difference in data distribution between each phase. Deep learning models underperformed overall, indicating the need for additional fine-tuning or integration with domain-specific adaptations to achieve comparable results. These findings suggest that ensemble methods combining the strengths of RF, XGBoost, and LR could improve overall performance. 
% Future work should investigate feature importance and conduct error analysis to identify misclassification patterns, guiding model refinement. 
% This table also underscores the need for a phase-aware modeling approach to optimize clinical trial outcome prediction.


% \begin{figure}[!t]
%     \centering
%     \includegraphics[width=0.85\linewidth,trim={0.5cm 2.5cm 0.5cm 0cm},clip]{figures/cto_method_2.pdf}
%     \caption{(A) provides the overview of the \method automated labeling framework. \method integrates various data sources to generate labels for predicting clinical trial outcomes. Data sources include (1) News articles, from which trial embeddings and sentiment scores are derived; (2) Publicly available stock prices, used to compute price changes before and after trials; (3) PubMed abstracts, where LLMs are prompted to predict the trial outcome; and (4) trial phase linkage. Additional sources of outcomes include trial metrics such as the number of patients, adverse events, etc. (B) Overview of trial linkage algorithm. (B1) Illustrates the phase connection map, covering all the phase categories present in the dataset. 
%     (B2) Linking trials across phases based on completion dates and intervention types, disease, and other trial data. We 1) constraint the search space, then 2) retrieve top-K most similar past trials using embeddings similarity. Finally, 3) a cross-encoder re-ranking strategy predicts linkages by scoring likely pairs.
%     (B3) Matching FDA-approved drugs from FDA orange book to Phase 3 and Phase 2 $\&$ 3 drug trials.}
%     \label{fig:trial_linkage} 
    
% \end{figure}


% \section*{\method\ Overview}
% \label{sec:overview}
% Our main methodology is outlined in Figure~\ref{fig:trial_linkage}A. We overview our primary sources of outcome predictors--LLM prediction on Pubmed Abstracts, Trial Linkage, News Headlines, Stock Price, and finally, Trial Metrics computed from clinicaltrials.gov. These metrics are computed independently and are aggregated via weakly supervised label aggregation.

% \subsection*{LLM Predictions on PubMed Abstracts}
% \label{sec:gpt}
% As many trials had multiple abstracts, we selected the top 2 abstracts based on their title similarity to the trial's official title to provide the most relevant information. Given these abstracts, we prompted the `GPT-3.5-turbo' model to summarize important trial-related statistical tests and predict the outcome. 
% % Additionally, we prompted the LLM to generate QA pairs about the trial, which are provided as a supplement ~\ref{supplementary: Additional Contributions} to our benchmark. The prompts are provided in the supplementary \ref{supplementary: Prompts for LLM Predictions}.

% % \textcolor{red}{Complete this section with more details}

% % For this section, we compute \andy{...Jathurshan, please complete --> done}

% \subsection*{Trial Linkage}
% \label{sec:linkage}
% The journey of a drug from discovery to FDA approval involves several stages, beginning with Phase 1 trials to assess safety and dosage. Subsequent Phase 2 and 3 trials evaluate efficacy and compare the new drug to existing therapies. Upon completing Phase 3, a drug may be submitted for FDA approval. A key limitation of the CTTI dataset is the lack of connectivity between trial phases, which could significantly enhance the ability to analyze trial progression and outcomes based on advancement to subsequent phases. Moreover, linking trials across phases is not straightforward due to challenges, including unstructured data, inconsistent reporting standards, missing information, data noise, and discrepancies in intervention details across phases. Despite these challenges, linking trials can be invaluable, particularly as a source of weak labels in clinical trial outcome prediction tasks. This section presents our novel trial-linking algorithm as illustrated in Figure~\ref{fig:trial_linkage}B, which, to our knowledge, is the first attempt to systematically connect different phases of clinical trials.
% The trial linkage extraction process consists of two primary steps: 1) Linking trials across different phases and 2) Matching phase 3 trials with FDA approvals (Figure~\ref{fig:trial_linkage}B3).

% The progression of clinical trials through phases is not all strictly sequential from Phase 1 to Phase 3, as some studies may combine multiple phases. Many trials were categorized as `Not Applicable' or were missing phase information entirely; these were excluded from our analysis. We created a phase connection map, illustrated in Figure~\ref{fig:trial_linkage}B1, that covers all phase categories present in the dataset. Our linking algorithm begins with the later phases and traces back to earlier phases.  This approach is based on the assumption that a trial in a subsequent phase implies the success and existence of a corresponding trial in a preceding phase. Phase 3 trials are considered a success if a Phase 4 trial is found or if it is linked to an FDA new drug application.

% The trial linkage process consists of three main steps: 1) Selection of the search space, 2) Retrieval of the top K most similar past trials, and 3) Prediction of linkage.  In Figure~\ref{fig:trial_linkage}B2, we illustrate an example of linking a Phase 4 trial to its preceding phases. For a given trial $x$, the objective is to identify its predecessor among trials in its directly linked earlier phases. For instance, the directly linked earlier phases of Phase 4 are Phase 3 and Phase 2$\&$3. 

% % \begin{figure}[t]
% %     \centering
% %     \includegraphics[width=\linewidth]{figures/Trial_Linking_Process2.pdf}
% %     \caption{Overview of trial linkage algorithm. A) Illustrates the phase connection map, covering all the phase categories present in the dataset. 
% %     B) Linking trials across phases based on completion dates and intervention types, disease, and other trial data. We 1) constraint the search space, then 2) retrieve top-K most similar past trials using embeddings similarity. Finally, 3) a cross-encoder re-ranking strategy predicts linkages by scoring likely pairs.
% %     C) Matching FDA-approved drugs from FDA orange book to Phase 3 and Phase 2 $\&$ 3 drug trials.}
% %     \label{fig:trial_linkage} 
% %     
% % \end{figure}



% \textbf{1. Search space selection:} We filter the trials based on their completion dates relative to the start date, ensuring that any linkage candidate must have concluded before the start of $x$. Furthermore, we also consider intervention types such as `Drug', `Biological', `Device', etc. 

% \textbf{2. Retrieve top-K:} From the filtered search space $\mathbf{Z}$, we retrieve top-32 most similar past trials to $x$. We extract key features and encode them into dense embedding using PubMedBERT \cite{gu2021domain} to represent both $x$ and trials in the search space ($z^i \in Z$) as follows: $x = \{x_{\text{I}},x_{\text{C}},x_{\text{T}},x_{\text{S}},x_{\text{E}}\}$,  $z^i =  \{z^i_{\text{I}},z^i_{\text{C}},z^i_{\text{T}},z^i_{\text{S}},z^i_{\text{E}}\}$.
% Where the subscript $I$ denotes intervention or drug, $C$ denotes condition or targeted disease, $T$ denotes official trial title, $S$ denotes trial summary, and $E$ denotes eligibility criteria. We calculate similarity as: $\text{similarity}(x^i,z^i) = \sum_{j \in \mathbf{F}}\frac{x^i \cdot z_j^i}{\|x^i\| \|z_j^i\|}
% $,
%     % \begin{equation}
%     %     \text{aggregated cos\_sim}(x,z^i) = \sum_{j \in \mathbf{F}}\frac{x^j.z^i^j}{||x^j||||z^i^j||}
%     % \end{equation}
% where $\mathbf{F} =$ \{I,C,T,S,E\}.
    
% We excluded the lead sponsor as a feature since the sponsor often changes depending on funding and performs worse empirically (See Supplementary: Ablation on Features for Trial Linkage).

% \textbf{3. Predict linkage} Given the large search space, we employ a re-ranking strategy using a cross-encoder pre-trained on MS-MARCO \cite{bajaj2016ms}. We provide feature pairs as input to the cross-encoder as follows: $\text{Cross-encoder score}(x^i,z^i) = \sum_{j \in \mathbf{F}}g_{\theta}(x^i,z^i_j)$.
%     % \begin{equation}
%     %     \text{Cross-encoder score}(x,z^i) = \sum_{j \in \mathbf{F}}g_{\theta}(x^j,z^j^i)
%     % \end{equation}
% Based on the cross-encoder scores, we predict the linkage by considering the trials with the highest positive cross-encoder scores as the most probable previous phase trials of $x$.

% We apply this process for all trials in Phase 4, Phase 3, Phase 2 \& 3, and Phase 2 to extract the trial linkages. To extract the outcome labels, we start with trials in the earlier phases and label them based on the existence of linked trials in the subsequent phases. However, trials in Phase 3 and Phase 4 have some exceptions to this process. For Phase 4 trials, there are no following trial phases, so we exclude them from the extracted weak labels. As for Phase 3 trials, they can be successful even without the existence of a subsequent Phase 4 trial. This highlights the importance of matching Phase 3 trials with their corresponding FDA approvals if they exist.

% After establishing connections across different phases of clinical trials, we focus on matching the Phase 3 trials to drug approvals to obtain their outcome labels. We utilize the FDA Orange Book\footnote{https://fda.gov/drugs/drug-approvals-and-databases/orange-book-data-files} version as of April 2024. Specifically, we use the approval date and drug name provided in the `product.txt' file, as the other files do not contain the relevant information required for the matching process. In this process, we only consider drug-related trials in Phase 3 and Phase 2 \& 3 since the Orange Book solely comprises FDA-approved drugs. 
% For a given FDA-approved drug, we first filter Phase 3 and Phase 2 \& 3 trials based on the approval date and intervention generic name, retaining trials completed between 2 years and 2 months prior to the approval date to align with the FDA approval process timeline. Similar to trial linkage prediction, we provide the drug's generic name and the trial's intervention generic name as input pairs to a cross-encoder, predicting their similarity. We select the top 5 trials based on cross-encoder scores and match the FDA approval to the trial with the completion date closest to the approval date. We then update the previously extracted outcomes for Phase 3 and Phase 2 \& 3 trials, labeling them as successful if matched to an FDA approval or having a linked Phase 4 trial.

% \subsection*{News Headlines}
% \label{sec:news}
% News headlines were obtained via the following steps: 
% % \begin{enumerate}
% We sent requests to Google News for all completed drug and biologic trials, which accounted for around 85k trials. Due to rate limitations, we utilize an external API (SerpAPI). We found that most trials do not have corresponding news--the total number of trials that had any corresponding news articles was 3688.

% % \jathu{Andy can you write up this section. Just add one or two sentence for completeness}
% We utilize Twitter-roBERTa-base for Sentiment Analysis \cite{loureiro2022timelms} to obtain sentiment (`Positive', `Negative', or `Neutral' with a confidence score between 0 and 1) for every headline.

% For the final labeling function prediction, we predicted 1 if the mode of all corresponding news was `Positive' or `Neutral', 0 if the mode was `Negative', and -1 (abstain) otherwise. From our perspective, if any news article was written about the trial, it should be relatively obvious if it was good or not. Often, news is written regarding trial plans or derivative results of a trial. In such cases, we make the assumption that such trials are more likely to be successful, as they are more ``exciting'' or are created from good results from a previous trial of the same drug.
% % We consider the mode of the news headlines as the predicted label.}

% % \end{enumerate}

% \subsection*{Stock Price} \label{sec:stock}
% % The stock price of a pharmaceutical or biotech company often reflects market expectations. If investors expect positive results, the stock may rise in anticipation of the trial's completion. Conversely, if expectations are low or if previous trials have been unsuccessful, the stock may not perform as well. We utilized Yahoo finance\footnote{\url{https://pypi.org/project/yfinance/}} to collect historical stock market data for companies that have publicly available tickers for completed trials. 
% In this section we provide more details on how the extracted stock price information is matched with the trials. By averaging the stock prices over a specified time frame, the moving average reduces the noise caused by random, short-term price movements, making it easier to identify the underlying trend \cite{investopedia_moving_average, schwab_momentum_indicator}. A 5-day simple moving average (SMA) of a stock's price is calculated by taking the average of the closing prices for the last 5 trading days. As shorter periods reveal shorter-term trends, we selected a 5-day SMA to capture the immediate short-term impact of the completion of clinical trials. A positive slope indicates an uptrend, while a negative slope indicates a downtrend in the SMA line \cite{schwab_momentum_indicator}. The absolute value of the slope represents the steepness of the trend. We calculated the slope for a 7-day window starting at a clinical trial's `completion date'. 

% \subsection*{Clinical Trial Metrics} 
% We utilize the CTTI dataset\footnote{\url{https://aact.ctti-clinicaltrials.org}} to obtain preprocessed tables of trial details (e.g. eligibility criteria, statistics, linked references \cite{califf2012characteristics,tasneem2012database,anderson2015compliance}.
% Specifically, we utilize the following information. (1) Whether results were reported, (2) The number of sponsors, (3) The number of patients, (4) The patient dropout rate, (5) The number of sites or locations for the trial, (6) Whether the P-value $<$ 0.05, (7) The date at which the trial was last updated vs its completion date, (8) Number of deaths, (9) Number of serious adverse events, (10) Number of \textit{any} adverse events, (11) The status of the trial e.g. terminated/withdrawn/completed/etc, and finally, (12) The number of amendments made to the trial page. Please see Weakly Supervised Labeling Functions in the Appendix for a discussion on how trial outcomes are linked to these metrics. 

% Each of these metrics is treated as a weakly supervised Labeling Function (LF). 
% For most of these metrics, we consider the "good" outcome as having greater or less than the median of that metric. For example, in the \textit{Serious Adverse Events LF}, we predict "1" if a trial's number of serious adverse events is less than the overall median number of serious adverse events. Otherwise, we predict "0". 
% While choosing a highly specific threshold could be better than choosing the median, we note that LFs in the data programming framework (as we describe in the next section) do not have to be perfect, only better than random for data programming to work well.

% % \subsection*{Labeling Pipeline}

% % % add status -> p-value -> label model (DP or RF)
% % % \subsubsection{Matrix Completion}
% % We design our clinical trial annotation pipeline by initially setting all terminated trials to 0. Next, trials with a primary outcome p-value $<$ 0.05 are set to 1. We then incorporate a label model to predict labels, leveraging multiple sources of weak supervision to identify highly confident predictions following an initial relation-prompting step.

% % A label model serves as the core framework here, producing denoised pseudo-labels by combining various weak supervision sources through labeling functions (LFs) and matrix completion \cite{ratner2016data, ratner2019training}. An LF is a heuristic that assigns labels to unlabeled data or abstains from labeling when uncertain. For instance, \texttt{f(trial) = return SUCCESS if p-value < 0.05 else ABSTAIN} 
% % is an LF for efficacy detection. More details are available in Appendix~\ref{app:dp}.

% % To validate our approach, we compare it with a \textit{Majority Vote} baseline--which simply assigns the mode prediction from all LFs, a Data Programming baseline--which unsupervised aggregates LFs, giving higher weight to LFs that agree with others, and finally, a supervised Random Forest baseline. Specifically, we train a Random Forest classifier to predict true labels from weakly supervised outputs, ensuring no data leakage by training solely on the training set of TOP.

% % Furthermore, we also humanly annotated more than 2500 hard samples that could be automatically determined as success or failure by p-value or the termination criterion. The result of our gold labels is shown in Figure~\ref{fig:human_labeled}. 













% % \section*{Appendix}
% % \label{sec:appendix}

% % % \clearpage
% % \section*{Additional Results and Contributions}
% % \subsection*{Results on TOP test data}
% % We run standard ML baselines \cite{fu2022hint}, namely Support Vector Machine (SVM), XGBoost, Multilayer Perceptron (MLP), Random Forest (RF), and Logistic Regression (LR). For these models, we model the trial outcome prediction task as a natural language classification task for maximum flexibility without requiring the need for molecular structure. TF-IDF is used to obtain features--the concatenated trial phase, disease indication, ICD codes, drugs, and eligibility criteria $\{x_{\text{P}}, x_{\text{I}},x_{\text{C}},x_{\text{T}},x_{\text{S}},x_{\text{E}}\}$. Essentially, we use the trial linkage features with the addition of Phase $x_{\text{P}}$. We additionally utilize PubMedBERT and BioBERT as additional baselines by adding an MLP classification head to the encoder output of the concatenated text.
% % The sizes of our train, validation, and test splits are 47080, 901, and 3165 respectively, with training and validation mined from \method\ (trials completed $<2014$ as per TOP \cite{fu2022hint}). We tested on the TOP test data. We demonstrate F1, PR-AUC, and ROC-AUC scores for all baseline models in Table \ref{tab:vstop_new}. 


% % We observe that models trained on \method's labels perform similarly, and even occasionally outperform those trained on supervised TOP. We hypothesize that this is due to a couple of factors. This demonstrates the effectiveness and reliability of our approach in predicting clinical trial outcomes. First, we combine highly diverse sources of LFs, the final predicted labels may serve as additional insights that the human annotators may have otherwise gleaned from fewer sources. Additionally, data programming enforces a level of self-regularization of the LFs, potentially smoothing the labels to allow for improved learning, much like in knowledge distillation's teacher pseudo-labels \cite{gou2021knowledge, hinton2015distilling}.

% % % Table~\ref{tab:vstop_new} presents a performance comparison of various models on the TOP test data split across different clinical trial phases (Phase 1, Phase 2, and Phase 3), with results shown for F1 score, PRAUC, and ROCAUC metrics. Our models, represented in red (\method), consistently achieve performance that is close to the baseline models represented in blue (TOP). Across all phases and metrics, the performance differences between \method\ and TOP are close, indicating that our models perform comparably well to the TOP baseline. This demonstrates the effectiveness and reliability of our approach in predicting clinical trial outcomes.

% % % \begin{figure}[ht]
% % %     \centering
% % %     \includegraphics[width=\linewidth]{figures/CTOD_vs_TOP_new.pdf}
% % %     \caption{Results on TOP test data split. The specific values can be found in Table~\ref{tab:vstop_new} in the Appendix. The average difference between TOP and \method\ is -0.007 F1 (\method\ actually improves F1 slightly on average), 0.018 PRAUC, and 0.022 ROCAUC.}
% % %     \label{fig:CTOD_vs_TOP_new} 
% % %     
% % % \end{figure}
% % \begin{table}[ht]
% % \centering
% % \caption{Comparison of baseline models trained on TOP vs \method\ labels. 
% % % The average difference between TOP and \method\ is -0.007 F1 (\method\ actually improves F1 slightly on average), 0.018 PRAUC, and 0.022 ROCAUC.
% % }
% % \label{tab:vstop_new}
% % \resizebox{\linewidth}{!}{
% % \LARGE
% % \begin{tabular}{ccccc|ccc|ccc}
% %  &  & \multicolumn{3}{c}{TOP} & \multicolumn{3}{c}{\method$_{RF}$} & \multicolumn{3}{c}{\method$_{DP}$} \\
% % Phase & Model & F1 & PRAUC & ROCAUC & F1 & PRAUC & ROCAUC & F1 & PRAUC & ROCAUC \\ \toprule
% % \multirow{9}{*}{I} & SVM & $0.632_{\pm0.019}$ & $0.645_{\pm0.028}$ & $0.592_{\pm0.023}$ & $0.713_{\pm0.015}$ & $0.661_{\pm0.027}$ & $0.626_{\pm0.021}$ & $0.720_{\pm0.010}$ & $0.648_{\pm0.017}$ & $0.614_{\pm0.013}$ \\
% %  & XGBoost & $0.630_{\pm0.020}$ & $0.637_{\pm0.025}$ & $0.596_{\pm0.021}$ & $0.706_{\pm0.017}$ & $0.675_{\pm0.030}$ & $0.645_{\pm0.021}$ & $0.719_{\pm0.016}$ & $0.656_{\pm0.027}$ & $0.606_{\pm0.023}$ \\
% %  & MLP & $0.585_{\pm0.023}$ & $0.636_{\pm0.028}$ & $0.575_{\pm0.022}$ & $0.661_{\pm0.019}$ & $0.645_{\pm0.026}$ & $0.600_{\pm0.018}$ & $0.655_{\pm0.020}$ & $0.626_{\pm0.030}$ & $0.581_{\pm0.024}$ \\
% %  & RF & $0.641_{\pm0.024}$ & $0.682_{\pm0.028}$ & $0.623_{\pm0.024}$ & $0.715_{\pm0.015}$ & $0.676_{\pm0.028}$ & $0.624_{\pm0.021}$ & $0.716_{\pm0.015}$ & $0.682_{\pm0.026}$ & $0.631_{\pm0.022}$ \\
% %  & LR & $0.656_{\pm0.018}$ & $0.669_{\pm0.028}$ & $0.631_{\pm0.021}$ & $0.715_{\pm0.016}$ & $0.690_{\pm0.029}$ & $0.656_{\pm0.023}$ & $0.726_{\pm0.016}$ & $0.693_{\pm0.029}$ & $0.660_{\pm0.021}$ \\
% %  & BioBERT & $0.627_{\pm0.022}$ & $0.665_{\pm0.029}$ & $0.612_{\pm0.023}$ & $0.713_{\pm0.015}$ & $0.676_{\pm0.019}$ & $0.641_{\pm0.020}$ & $0.716_{\pm0.016}$ & $0.677_{\pm0.019}$ & $0.649_{\pm0.015}$ \\
% %  & PubMedBERT & $0.646_{\pm0.014}$ & $0.602_{\pm0.017}$ & $0.588_{\pm0.015}$ & $0.715_{\pm0.014}$ & $0.595_{\pm0.018}$ & $0.579_{\pm0.013}$ & $0.719_{\pm0.015}$ & $0.591_{\pm0.020}$ & $0.571_{\pm0.012}$ \\
% %  & HINT & $0.621_{\pm0.022}$ & $0.633_{\pm0.029}$ & $0.590_{\pm0.025}$ & $0.611_{\pm0.020}$ & $0.559_{\pm0.022}$ & $0.520_{\pm0.031}$ & $0.607_{\pm0.021}$ & $0.490_{\pm0.035}$ & $0.545_{\pm0.026}$ \\
% %  & SPOT & $0.652_{\pm0.025}$ & $0.679_{\pm0.029}$ & $0.624_{\pm0.028}$ & $0.600_{\pm0.016}$ & $0.670_{\pm0.022}$ & $0.635_{\pm0.016}$ & $0.625_{\pm0.029}$ & $0.693_{\pm0.026}$ & $0.646_{\pm0.027}$ \\ \midrule
% % \multirow{9}{*}{II} & SVM & $0.672_{\pm0.011}$ & $0.664_{\pm0.017}$ & $0.626_{\pm0.013}$ & $0.715_{\pm0.010}$ & $0.653_{\pm0.017}$ & $0.617_{\pm0.012}$ & $0.720_{\pm0.010}$ & $0.648_{\pm0.017}$ & $0.614_{\pm0.013}$ \\
% %  & XGBoost & $0.659_{\pm0.013}$ & $0.675_{\pm0.016}$ & $0.627_{\pm0.014}$ & $0.706_{\pm0.011}$ & $0.650_{\pm0.018}$ & $0.609_{\pm0.014}$ & $0.710_{\pm0.012}$ & $0.644_{\pm0.018}$ & $0.607_{\pm0.014}$ \\
% %  & MLP & $0.615_{\pm0.014}$ & $0.640_{\pm0.017}$ & $0.599_{\pm0.014}$ & $0.671_{\pm0.011}$ & $0.638_{\pm0.017}$ & $0.601_{\pm0.015}$ & $0.673_{\pm0.012}$ & $0.647_{\pm0.017}$ & $0.599_{\pm0.013}$ \\
% %  & RF & $0.675_{\pm0.011}$ & $0.690_{\pm0.016}$ & $0.643_{\pm0.014}$ & $0.715_{\pm0.010}$ & $0.671_{\pm0.017}$ & $0.628_{\pm0.013}$ & $0.712_{\pm0.011}$ & $0.657_{\pm0.018}$ & $0.623_{\pm0.014}$ \\
% %  & LR & $0.674_{\pm0.013}$ & $0.697_{\pm0.017}$ & $0.648_{\pm0.012}$ & $0.714_{\pm0.010}$ & $0.686_{\pm0.017}$ & $0.646_{\pm0.015}$ & $0.718_{\pm0.010}$ & $0.679_{\pm0.016}$ & $0.642_{\pm0.014}$ \\
% %  & BioBERT & $0.672_{\pm0.016}$ & $0.696_{\pm0.025}$ & $0.648_{\pm0.015}$ & $0.715_{\pm0.007}$ & $0.674_{\pm0.014}$ & $0.642_{\pm0.014}$ & $0.718_{\pm0.007}$ & $0.657_{\pm0.014}$ & $0.627_{\pm0.014}$ \\
% %  & PubMedBERT & $0.682_{\pm0.010}$ & $0.612_{\pm0.010}$ & $0.601_{\pm0.009}$ & $0.705_{\pm0.009}$ & $0.578_{\pm0.010}$ & $0.545_{\pm0.010}$ & $0.713_{\pm0.009}$ & $0.575_{\pm0.010}$ & $0.540_{\pm0.006}$ \\
% %  & HINT & $0.654_{\pm0.013}$ & $0.680_{\pm0.016}$ & $0.632_{\pm0.013}$ & $0.708_{\pm0.010}$ & $0.647_{\pm0.018}$ & $0.627_{\pm0.014}$ & $0.713_{\pm0.007}$ & $0.670_{\pm0.013}$ & $0.635_{\pm0.016}$ \\
% %  & SPOT & $0.681_{\pm0.009}$ & $0.660_{\pm0.012}$ & $0.617_{\pm0.010}$ & $0.601_{\pm0.014}$ & $0.666_{\pm0.020}$ & $0.625_{\pm0.014}$ & $0.608_{\pm0.015}$ & $0.677_{\pm0.017}$ & $0.622_{\pm0.014}$ \\ \midrule
% % \multirow{9}{*}{III} & SVM & $0.813_{\pm0.010}$ & $0.876_{\pm0.012}$ & $0.700_{\pm0.018}$ & $0.853_{\pm0.009}$ & $0.859_{\pm0.013}$ & $0.674_{\pm0.017}$ & $0.854_{\pm0.007}$ & $0.840_{\pm0.014}$ & $0.653_{\pm0.018}$ \\
% %  & XGBoost & $0.815_{\pm0.010}$ & $0.849_{\pm0.015}$ & $0.674_{\pm0.017}$ & $0.852_{\pm0.009}$ & $0.848_{\pm0.014}$ & $0.666_{\pm0.018}$ & $0.855_{\pm0.008}$ & $0.846_{\pm0.013}$ & $0.659_{\pm0.018}$ \\
% %  & MLP & $0.762_{\pm0.011}$ & $0.848_{\pm0.012}$ & $0.650_{\pm0.017}$ & $0.824_{\pm0.011}$ & $0.856_{\pm0.011}$ & $0.666_{\pm0.016}$ & $0.833_{\pm0.009}$ & $0.839_{\pm0.013}$ & $0.642_{\pm0.021}$ \\
% %  & RF & $0.830_{\pm0.009}$ & $0.858_{\pm0.013}$ & $0.675_{\pm0.015}$ & $0.857_{\pm0.008}$ & $0.844_{\pm0.014}$ & $0.656_{\pm0.018}$ & $0.857_{\pm0.009}$ & $0.831_{\pm0.014}$ & $0.639_{\pm0.017}$ \\
% %  & LR & $0.828_{\pm0.008}$ & $0.887_{\pm0.010}$ & $0.725_{\pm0.014}$ & $0.855_{\pm0.008}$ & $0.870_{\pm0.013}$ & $0.705_{\pm0.017}$ & $0.857_{\pm0.008}$ & $0.847_{\pm0.013}$ & $0.677_{\pm0.019}$ \\
% %  & BioBERT & $0.838_{\pm0.009}$ & $0.859_{\pm0.012}$ & $0.696_{\pm0.016}$ & $0.854_{\pm0.010}$ & $0.681_{\pm0.015}$ & $0.848_{\pm0.014}$ & $0.855_{\pm0.010}$ & $0.833_{\pm0.013}$ & $0.650_{\pm0.015}$ \\
% %  & PubMedBERT & $0.850_{\pm0.008}$ & $0.809_{\pm0.014}$ & $0.650_{\pm0.013}$ & $0.852_{\pm0.010}$ & $0.759_{\pm0.015}$ & $0.531_{\pm0.008}$ & $0.855_{\pm0.010}$ & $0.756_{\pm0.016}$ & $0.522_{\pm0.004}$ \\
% %  & HINT & $0.825_{\pm0.009}$ & $0.850_{\pm0.016}$ & $0.696_{\pm0.017}$ & $0.872_{\pm0.006}$ & $0.830_{\pm0.017}$ & $0.592_{\pm0.020}$ & $0.871_{\pm0.006}$ & $0.828_{\pm0.012}$ & $0.606_{\pm0.014}$ \\
% %  & SPOT & $0.832_{\pm0.008}$ & $0.862_{\pm0.013}$ & $0.676_{\pm0.020}$ & $0.676_{\pm0.015}$ & $0.834_{\pm0.016}$ & $0.665_{\pm0.018}$ & $0.653_{\pm0.013}$ & $0.834_{\pm0.015}$ & $0.638_{\pm0.016}$
% % \end{tabular}
% % }
% % \end{table}
% % % \andy{insert barplot figure here with updated results, note that weak labels sometimes perform better than HINT}


% % \subsection*{Results on Pre-2020 Split vs Post-2020 Split} 

% % Since Covid changed the landscape of clinical trials due to its disruptive nature, the trial distribution before and after 2020 are quite different (See empirical performance in Table~\ref{tab:prevspost_dp}). Note that we choose \method$_{DP}$, since despite its lower performance on TOP, we believe it has stronger generalizability to all trials, as shown by its proportion of positive and negative outcome label prediction in Figure~\ref{fig:final_label_stats}.

% % The \textit{Pre-2020 Split} consists of trials where their completion dates are before 2018. The test completion dates start in 2018 but are within 2020. This split has 27,245, 6,828, and 6,151 samples in the training, validation, and test sets, respectively. We have another data split, the \textit{Post-2020 Split}. The completion dates of the training trials are before 2020, while the test completion dates are after 2020 but before 2024. This split has 32,200, 8,024, and 12,525 samples in the training, validation, and test sets, respectively. 

% % Note that for post-2020, the training set includes all trials that were completed before 2020 and therefore the entire Pre-2020 dataset.

% % We additionally show results from both pre- and post-2020 splits in Table~\ref{tab:prevspost_dp}. The pre-2020 split shows generally higher performance across all metrics and phases compared to the post-2020 split, indicating that the pre-2020 data is easier to predict. The decline in performance post-2020 can be attributed to the complexities and disruptions introduced by the COVID-19 pandemic, which affected clinical trial operations and outcomes. Overall, these observations suggest that the pre-2020 data offers a more stable and predictable environment for clinical trial outcome prediction and that post-2020 data should require additional consideration.

% % \begin{table}[ht]
% % \centering
% % \caption{Performance of baselines on both data splits of \method\ for \method$_{DP}$. The average difference for pre- and post-2020 is 0.035 F1, 0.056 PRAUC, and 0.029 ROCAUC.}
% % \label{tab:prevspost_dp}
% % \resizebox{\linewidth}{!}{
% % \begin{tabular}{ccccc|ccc}
% %  &  & \multicolumn{3}{c}{Pre} & \multicolumn{3}{c}{Post} \\
% % Phase & Model & F1 & PRAUC & ROCAUC & F1 & PRAUC & ROCAUC \\ \toprule
% % \multirow{7}{*}{I} & SVM & $0.744_{\pm0.008}$ & $0.632_{\pm0.015}$ & $0.556_{\pm0.012}$ & $0.664_{\pm0.007}$ & $0.516_{\pm0.012}$ & $0.528_{\pm0.010}$ \\
% %  & XGBoost & $0.731_{\pm0.008}$ & $0.656_{\pm0.013}$ & $0.561_{\pm0.012}$ & $0.646_{\pm0.007}$ & $0.532_{\pm0.012}$ & $0.545_{\pm0.009}$ \\
% %  & MLP & $0.673_{\pm0.010}$ & $0.614_{\pm0.016}$ & $0.545_{\pm0.015}$ & $0.583_{\pm0.009}$ & $0.518_{\pm0.011}$ & $0.532_{\pm0.009}$ \\
% %  & RF & $0.744_{\pm0.008}$ & $0.591_{\pm0.014}$ & $0.502_{\pm0.011}$ & $0.662_{\pm0.006}$ & $0.468_{\pm0.009}$ & $0.458_{\pm0.009}$ \\
% %  & LR & $0.740_{\pm0.008}$ & $0.628_{\pm0.015}$ & $0.548_{\pm0.012}$ & $0.651_{\pm0.007}$ & $0.505_{\pm0.011}$ & $0.519_{\pm0.009}$ \\
% %  & PubMedBERT & $0.743_{\pm0.005}$ & $0.623_{\pm0.017}$ & $0.538_{\pm0.016}$ & $0.664_{\pm0.006}$ & $0.511_{\pm0.008}$ & $0.527_{\pm0.005}$ \\
% %  & BioBERT & $0.743_{\pm0.005}$ & $0.613_{\pm0.014}$ & $0.522_{\pm0.014}$ & $0.664_{\pm0.006}$ & $0.476_{\pm0.009}$ & $0.490_{\pm0.008}$ \\ \midrule
% % \multirow{7}{*}{II} & SVM & $0.862_{\pm0.005}$ & $0.795_{\pm0.011}$ & $0.574_{\pm0.012}$ & $0.849_{\pm0.003}$ & $0.781_{\pm0.007}$ & $0.569_{\pm0.009}$ \\
% %  & XGBoost & $0.843_{\pm0.005}$ & $0.810_{\pm0.009}$ & $0.582_{\pm0.012}$ & $0.820_{\pm0.004}$ & $0.775_{\pm0.008}$ & $0.559_{\pm0.008}$ \\
% %  & MLP & $0.784_{\pm0.006}$ & $0.790_{\pm0.010}$ & $0.569_{\pm0.012}$ & $0.750_{\pm0.005}$ & $0.765_{\pm0.007}$ & $0.545_{\pm0.008}$ \\
% %  & RF & $0.863_{\pm0.005}$ & $0.799_{\pm0.009}$ & $0.574_{\pm0.011}$ & $0.850_{\pm0.004}$ & $0.762_{\pm0.008}$ & $0.532_{\pm0.009}$ \\
% %  & LR & $0.856_{\pm0.006}$ & $0.797_{\pm0.009}$ & $0.579_{\pm0.010}$ & $0.835_{\pm0.004}$ & $0.779_{\pm0.007}$ & $0.568_{\pm0.008}$ \\
% %  & PubMedBERT & $0.865_{\pm0.004}$ & $0.812_{\pm0.009}$ & $0.583_{\pm0.012}$ & $0.849_{\pm0.004}$ & $0.741_{\pm0.005}$ & $0.508_{\pm0.005}$ \\
% %  & BioBERT & $0.865_{\pm0.004}$ & $0.829_{\pm0.010}$ & $0.603_{\pm0.012}$ & $0.849_{\pm0.004}$ & $0.779_{\pm0.007}$ & $0.563_{\pm0.008}$ \\ \midrule
% % \multirow{7}{*}{III} & SVM & $0.910_{\pm0.005}$ & $0.863_{\pm0.011}$ & $0.560_{\pm0.020}$ & $0.912_{\pm0.003}$ & $0.864_{\pm0.007}$ & $0.563_{\pm0.011}$ \\
% %  & XGBoost & $0.901_{\pm0.006}$ & $0.867_{\pm0.010}$ & $0.574_{\pm0.020}$ & $0.894_{\pm0.004}$ & $0.858_{\pm0.009}$ & $0.552_{\pm0.015}$ \\
% %  & MLP & $0.841_{\pm0.008}$ & $0.851_{\pm0.012}$ & $0.551_{\pm0.017}$ & $0.825_{\pm0.005}$ & $0.846_{\pm0.010}$ & $0.523_{\pm0.014}$ \\
% %  & RF & $0.910_{\pm0.005}$ & $0.856_{\pm0.011}$ & $0.536_{\pm0.019}$ & $0.912_{\pm0.003}$ & $0.854_{\pm0.007}$ & $0.529_{\pm0.014}$ \\
% %  & LR & $0.906_{\pm0.006}$ & $0.870_{\pm0.013}$ & $0.576_{\pm0.017}$ & $0.904_{\pm0.004}$ & $0.860_{\pm0.008}$ & $0.561_{\pm0.013}$ \\
% %  & PubMedBERT & $0.911_{\pm0.004}$ & $0.878_{\pm0.009}$ & $0.598_{\pm0.016}$ & $0.911_{\pm0.003}$ & $0.836_{\pm0.004}$ & $0.497_{\pm0.006}$ \\
% %  & BioBERT & $0.911_{\pm0.004}$ & $0.892_{\pm0.011}$ & $0.631_{\pm0.019}$ & $0.911_{\pm0.003}$ & $0.870_{\pm0.005}$ & $0.585_{\pm0.012}$ \\ \bottomrule
% % \end{tabular}
% % }
% % \end{table}



% % \subsection*{Additional Contributions}
% % \label{supplementary: Additional Contributions}
% % % \andy{potential Appendix}

% % \paragraph{Additional Feature Collection}
% % To run the baselines, we needed to collect ICD codes for diseases and SMILES strings \cite{weininger1988smiles} for drugs. We collected \textbf{ICD10 codes} for the diseases from the NIH Clinical Table Search Service\footnote{\url{https://clinicaltables.nlm.nih.gov/}}\cite{fu2022hint}. 
% % % We slightly modified their code from \url{https://github.com/futianfan/clinical-trial-outcome-prediction/blob/main/benchmark/disease2icd.py} to accommodate cases that HINT cannot handle.
% % We additionally collected \textbf{SMILES} (Simplified Molecular Input Line Entry System) strings for drugs from DrugBank 
% % % \url{https://go.drugbank.com/releases/latest}. 
% % We also used NIH PubChem\footnote{PubChemPy API \url{https://pubchempy.readthedocs.io/en/latest/}} \cite{kim2018update, kim2015pug, kim2019programmatic} to collect the SMILES we could not find in DrugBank.

% % \paragraph{Stock Trend Prediction} \label{stock_trend}
% % The trend of a stock price is the overall direction in which the price of the stock is moving over a specified period, derived from the historical price data \cite{fidelity_trend}. As discussed in \ref{sec:stock}, we calculated the slope of stock prices. We define trend as the direction of the slope, i.e., positive slope refers to positive trend, and negative slope refers to negative trend. We tried to predict the trend of stock price in the 7-day window starting from a clinical trial's completion date.  Table \ref{tab:stockpred} shows the scores for different ML models for stock trend prediction. We utilized phase, eligibility criteria, diseases, and drugs as features for predicting trend. We get embeddings of the features using BioBERT and use the embeddings as input to the different baseline methods of Table \ref{tab:stockpred}. 

% % % \begin{wraptable}{R}{.3\linewidth}
% % % \vspace{-1.25em}
% % \begin{table}[ht]
% % \centering
% % % \setlength{\tabcolsep}{1pt}
% % \caption{Comparison of model performance metrics for stock trend prediction}
% % \label{tab:stockpred}
% % % \resizebox{\linewidth}{!}{
% % % \Huge
% % \begin{tabular}{ccccccc}
% %     Model & Accuracy & ROCAUC & F1 \\
% %     \toprule
% %     LR & 0.5121 & 0.5314 & 0.5531  \\
% %     MLP               & 0.5418 & 0.5202 & 0.6620  \\
% %     SVM                & 0.5441 & 0.4878 & 0.6860 \\
% %     RF      & 0.5040 & 0.5103 & 0.5377  \\
% %     XGBoost            & 0.5013 & 0.5077 & 0.5340 \\
% %     \bottomrule
% % \end{tabular}
% % % }
% % \end{table}

% % % 
% % % \end{wraptable} 

% % \paragraph{QA Dataset}\label{QA}

% % In addition to the weak trial outcome labels, we provide a QA dataset on trial publications as an additional contribution. While obtaining LLM predictions on PubMed abstracts, we prompted the model to generate question-answer pairs from the given abstracts. The prompts for generating the QA pairs are provided in the supplementary material (Figure~\ref{fig:LLM_prompts}). The answers are provided in both short-answer and multiple-choice formats. Examples can be found in the supplementary material (Fig~\ref{fig:GPT_response example} and ~\ref{fig:GPT_response example2}). This QA dataset offers valuable information about the trials, complementing the weak outcome labels. It can be used for various downstream tasks, such as question answering, information extraction, and knowledge base construction related to clinical trials.


% % % \subsection*{Additional Tables}
% % % This shows all results for both 

% % % \clearpage

% % % \subsection*{Results on TOP (All Drugs)}
% % % \label{app:top_extended}

% % % In this section, we run comparisons of an extended training set--now selecting all interventional small molecule drug trials with completion dates before 2014. The sizes of our train, validation, and test splits are 47,080, 901, and 3165 respectively, with training and validation mined from \method\ (trials completed $<2014$ as per TOP \cite{fu2022hint}). We tested on the TOP test data. We demonstrate F1, PR-AUC, and ROC-AUC scores for all baseline models in table \ref{tab:vstop}. 
% % % % \subsection*{Baselines}
% % % \begin{figure}[ht]
% % %     \centering
% % %     \includegraphics[width=\linewidth]{figures/CTOD_vs_TOP_old.pdf}
% % %     \caption{Results on TOP test data split. The specific values can be found in Table~\ref{tab:vstop} in the Appendix. The average difference between TOP and \method\ is 0.048 F1,  0.077 PRAUC, and 0.098 ROCAUC.}
% % %     \label{fig: CTOD vs TOP} 
% % %     
% % % \end{figure}

% % % \begin{table}[ht]
% % % \centering
% % % \caption{On TOP. Train/Valid/Test split is 47,080 / 901 / 3,165. The average difference between TOP and \method\ is 0.048 F1,  0.077 PRAUC, and 0.098 ROCAUC.}
% % % \label{tab:vstop}
% % % \resizebox{\linewidth}{!}{
% % % \begin{tabular}{ccccc|ccc}
% % %  &  & \multicolumn{3}{c}{TOP} & \multicolumn{3}{c}{CTO} \\
% % % Phase & Model & F1 & PRAUC & ROCAUC & F1 & PRAUC & ROCAUC \\ \toprule
% % % \multirow{7}{*}{I} & SVM & $0.632_{\pm0.019}$ & $0.645_{\pm0.028}$ & $0.592_{\pm0.023}$ & $0.563_{\pm0.019}$ & $0.608_{\pm0.026}$ & $0.529_{\pm0.019}$ \\
% % %  & XGBoost & $0.630_{\pm0.020}$ & $0.637_{\pm0.025}$ & $0.596_{\pm0.021}$ & $0.586_{\pm0.021}$ & $0.584_{\pm0.024}$ & $0.527_{\pm0.024}$ \\
% % %  & MLP & $0.585_{\pm0.023}$ & $0.636_{\pm0.028}$ & $0.575_{\pm0.022}$ & $0.566_{\pm0.022}$ & $0.594_{\pm0.024}$ & $0.529_{\pm0.022}$ \\
% % %  & RF & $0.641_{\pm0.024}$ & $0.682_{\pm0.028}$ & $0.623_{\pm0.024}$ & $0.528_{\pm0.022}$ & $0.558_{\pm0.024}$ & $0.492_{\pm0.023}$ \\
% % %  & LR & $0.656_{\pm0.018}$ & $0.669_{\pm0.028}$ & $0.631_{\pm0.021}$ & $0.584_{\pm0.021}$ & $0.613_{\pm0.030}$ & $0.529_{\pm0.024}$ \\
% % %  & BioBERT & $0.653_{\pm0.017}$ & $0.674_{\pm0.014}$ & $0.622_{\pm0.021}$ & $0.567_{\pm0.023}$ & $0.563_{\pm0.023}$ & $0.504_{\pm0.027}$ \\
% % %  & PubMedBERT & $0.597_{\pm0.017}$ & $0.609_{\pm0.016}$ & $0.596_{\pm0.019}$ & $0.593_{\pm0.027}$ & $0.572_{\pm0.023}$ & $0.528_{\pm0.025}$ \\ \midrule
% % % \multirow{7}{*}{II} & SVM & $0.672_{\pm0.011}$ & $0.664_{\pm0.017}$ & $0.626_{\pm0.013}$ & $0.613_{\pm0.013}$ & $0.578_{\pm0.017}$ & $0.529_{\pm0.014}$ \\
% % %  & XGBoost & $0.659_{\pm0.013}$ & $0.675_{\pm0.016}$ & $0.627_{\pm0.014}$ & $0.598_{\pm0.014}$ & $0.565_{\pm0.020}$ & $0.512_{\pm0.015}$ \\
% % %  & MLP & $0.615_{\pm0.014}$ & $0.640_{\pm0.017}$ & $0.599_{\pm0.014}$ & $0.611_{\pm0.012}$ & $0.595_{\pm0.018}$ & $0.542_{\pm0.015}$ \\
% % %  & RF & $0.675_{\pm0.011}$ & $0.690_{\pm0.016}$ & $0.643_{\pm0.014}$ & $0.574_{\pm0.014}$ & $0.539_{\pm0.017}$ & $0.475_{\pm0.014}$ \\
% % %  & LR & $0.674_{\pm0.013}$ & $0.697_{\pm0.017}$ & $0.648_{\pm0.012}$ & $0.626_{\pm0.012}$ & $0.579_{\pm0.017}$ & $0.528_{\pm0.013}$ \\
% % %  & BioBERT & $0.669_{\pm0.014}$ & $0.694_{\pm0.017}$ & $0.647_{\pm0.010}$ & $0.611_{\pm0.001}$ & $0.574_{\pm0.017}$ & $0.508_{\pm0.011}$ \\
% % %  & PubMedBERT & $0.644_{\pm0.009}$ & $0.612_{\pm0.008}$ & $0.600_{\pm0.010}$ & $0.595_{\pm0.011}$ & $0.561_{\pm0.013}$ & $0.509_{\pm0.010}$ \\ \midrule
% % % \multirow{7}{*}{III} & SVM & $0.813_{\pm0.010}$ & $0.876_{\pm0.012}$ & $0.700_{\pm0.018}$ & $0.788_{\pm0.010}$ & $0.782_{\pm0.015}$ & $0.595_{\pm0.021}$ \\
% % %  & XGBoost & $0.815_{\pm0.010}$ & $0.849_{\pm0.015}$ & $0.674_{\pm0.017}$ & $0.789_{\pm0.010}$ & $0.799_{\pm0.017}$ & $0.597_{\pm0.019}$ \\
% % %  & MLP & $0.762_{\pm0.011}$ & $0.848_{\pm0.012}$ & $0.650_{\pm0.017}$ & $0.769_{\pm0.011}$ & $0.780_{\pm0.016}$ & $0.559_{\pm0.020}$ \\
% % %  & RF & $0.830_{\pm0.009}$ & $0.858_{\pm0.013}$ & $0.675_{\pm0.015}$ & $0.746_{\pm0.011}$ & $0.782_{\pm0.017}$ & $0.562_{\pm0.020}$ \\
% % %  & LR & $0.828_{\pm0.008}$ & $0.887_{\pm0.010}$ & $0.725_{\pm0.014}$ & $0.802_{\pm0.011}$ & $0.782_{\pm0.019}$ & $0.592_{\pm0.020}$ \\
% % %  & BioBERT & $0.832_{\pm0.010}$ & $0.850_{\pm0.016}$ & $0.662_{\pm0.018}$ & $0.791_{\pm0.012}$ & $0.808_{\pm0.022}$ & $0.592_{\pm0.025}$ \\
% % %  & PubMedBERT & $0.824_{\pm0.009}$ & $0.808_{\pm0.015}$ & $0.646_{\pm0.014}$ & $0.791_{\pm0.013}$ & $0.774_{\pm0.013}$ & $0.565_{\pm0.021}$ \\ \bottomrule
% % % \end{tabular}
% % % }
% % % \end{table}

% % % We see that from Table~\ref{tab:vstop} and Figure~\ref{fig: CTOD vs TOP} that our data is still close. However, SPOT and HINT perform quite badly on the extended dataset. We hypothesize that this is because both these models, due to their complexity tend to overfit to the TOP train split. However, simple baselines such as SVM and LR simply cannot overfit, and therefore better preserve the generalizability. Further investigation is required to fully analyze the distribution shift between the TOP training set and the set of all interventional drug trials.

% % % % \andy{add bad SPOT AND HINT results here}

% % % \clearpage

% \section*{Label Creation Continued}

% \subsection*{Data Programming}
% \label{app:dp}
% The full data programming framework is detailed by Ratner et al. \cite{ratner2019training}. We introduce a small aspect of the framework below.
% At a high level, the aggregation of weakly supervised labeling functions (LFs) is framed as a dependency graph $G_{source}$ where each LF $\lambda_i$ is dependently conditioned on the true label $Y$. In our case, we assume conditional independence of all $\lambda_i | Y$. For this case, the dependency graphs will have observable cliques  $\bm{O} = \{\lambda_i, i \in n_{lf}\} \subset C$, where $n_{lf}$ is the number of labeling functions.

% From here, the covariance matrix of an observable subset of the cliques in $G_{source}$ is analyzed, leading to a matrix completion approach for recovering estimated accuracies $\mu$ (used in the final label model to predict $P(\bm{Y}|\bm{\lambda})$).

% Let $\mu = \mathbb{E}(\psi(C))$ where $\psi(C)$ is a vector of indicator random variables for all combinations of all but one of the labels emitted by each variable in clique C.

% The norm of the covariance of observed LFs cliques $O$ and separator set $S$ cliques $\bm{Cov}(\psi(O) \cup \psi(S))$ can be used to recover $\mu$. 

% \begin{align}
% & \bm{Cov}(\psi(O) \cup \psi(S)) = \Sigma =  \begin{bmatrix}
% \Sigma_{O} & \Sigma_{OS} \\
% \Sigma_{OS}^T & \Sigma_{S}
% \end{bmatrix}
% \end{align}
% Its inverse is:
% \begin{align}
% & K = \Sigma^{-1} =  \begin{bmatrix}
% K_{O} & K_{OS} \\
% K_{OS}^T & K_{S}
% \end{bmatrix}
% \end{align}
% Applying block matrix inversion, we get:
% $$K_O = \Sigma^{-1}_O + c \Sigma^{-1}_O \Sigma_{OS} \Sigma^T_{OS} \Sigma^{-1}_{O}$$
% $$c = (\Sigma_{S} - \Sigma^T_{OS} \Sigma^{-1}_{O} \Sigma_{OS})$$
% Let $z = \sqrt{z} \Sigma^{-1}_{O} \Sigma_{OS}$, then
% $$K_O = \Sigma^{-1}_O + zz^T$$
% Solving for $z$ can directly recover estimated accuracies from $\mu$ via Algorithm 1 in Ratner et al. \cite{ratner2019training}.

% % \subsection*{Case Studies}
% % In this section, we will analyze a few of the predicted differences between TOP and CTOD.

% % \subsection*{LLM Prompts}

% \subsection*{Weakly Supervised Labeling Functions}
% \label{app:metrics}
% In this section, we report all of our LFs and their implementations.

% \begin{itemize}
% \item \texttt{results\_reported}: 1 if results were reported for a trial. Otherwise, it predicts 0. 

% \item \texttt{num\_sponsors}: The number of sponsors for a trial. Can be thresholded.  It is important to study the impact of single sponsors, multiple sponsors, collaborative partnerships, and public funding. The number and type of sponsors will have a significant impact on the clinical trial process and the overall path of bringing the new drug to market. Sponsors affect all parts of the trial, from funding and resources, regulatory guidance, global reach, operational support, supply chain management, market access and distribution, and risk management.  

% \item \texttt{num\_patients}: The number of patients for a trial. Can be thresholded. As the clinical trials are conducted with strong statistical power to detect the true effect of the drug and to minimize the risk of committing Type II error (failing to detect the treatment effect that is present or false negatives), number of participants in each respective trial is key aspect of trial success.

% \item \texttt{patient\_drop}: The number of patients that drop out during the trial. Can be thresholded. Patients drop out from the clinical trial due to lack of efficacy unintended adverse events or other reasons that could result in unanticipated trial outcomes. 

% \item \texttt{sites}: The number of total sites during the trial. Can be thresholded. This also indirectly measures the funding capabilities of the sponsors, much like num\_sponsors.

% \item \texttt{pvalues}: Whether there exists a primary outcome P-value $<$ 0.05. If there is at least one significant result, we consider this a success. Otherwise, we predict failure.

% \item \texttt{update\_more\_recent}: The difference in the date at which the trial was last updated vs its completion date. Can be thresholded. The time gap can provide critical insights into the trials' post-completion process and transparency. Identifying delays is helpful for trial success, as it could be due to data analysis and validation, regulatory review, and publication process. A highly amended trial could indicate success due to the large amount of publications.

% \item \texttt{death\_ae, serious\_ae, all\_ae}: Represents the number of deaths, serious adverse events, and total adverse events, respectively. Can be thresholded. The total number of adverse events (AEs), serious adverse events (SAEs), and deaths in a clinical trial can provide important safety information about the investigational treatment. However, the significance of these numbers depends on various factors, including the size and duration of the trial, the nature of the treatment, and the characteristics of the study population. 
% % Understanding the safety, tolerability, and risk-benefit profile of investigational products will guide decisions on dose optimization, patient selection, safety monitoring strategies, and regulatory strategies with a focus on clinical trial participant safety. 

% \item \texttt{status}: The status of the trial. We say that a trial is not successful if the status is \textit{'Terminated', 'Withdrawn', 'Suspended', 'Withheld', 'No longer available', or 'Temporarily not available'}. However, if it is \textit{'Approved for marketing'}, then we say it is successful. Otherwise, we abstain from predicting either. Having this information incorporated serves to enhance the transparency, regulatory compliance, and ethical conduct of clinical trials. I.e. \textit{"Terminated: The study has stopped early and will not start again. Participants are no longer being examined or treated."} usually occurs when the trial causes significant negative side-effects in several patients.

% \item \texttt{amendments}: Represents the number of trial amendments. Can be thresholded.
% Clinical trials must follow approved protocols \cite{ICH2016, MHRA2012}, but amendments may be required after regulatory approval to adjust protocols according to new requirements or insights. 
% We scraped record histories for each trial from \url{https://clinicaltrials.gov/} and calculated the total number of times a clinical trial has been amended. The number of amendments to a clinical trial protocol can provide some insights into the trial's progress and potential success, but it's not necessarily a direct indication of success or failure. Therefore, we consider the total number of amendments of trial as a weak label. Sometimes, amendments to trial protocols are crucial for adapting to emerging data from ongoing clinical trials, addressing safety concerns, or optimizing study design to yield better outcomes. 

% \item \texttt{stock\_price}: Is positive if the sponsor stock price's 5-day moving average has a positive or negative slope. 

% \item \texttt{linkage}: Is positive if a trial was found to have any later-stage trials linked to it.

% \item \texttt{news\_headlines}: Is positive or negative depending on sentiment from any news headline related to the trial.

% \item \texttt{gpt}: Represents GPT3.5-turbo-0125's decisions on PubMed abstracts.

% \end{itemize}

% \subsection*{Phase-Specific Thresholding}
% For Phases 1, 2, and 3, we find specific quantile thresholds from $(0.1, 0.2, ..., 0.9)$ for all LFs that have tunable thresholds, fine-tuned on each respective phase on the TOP training dataset.

% To reiterate our final labeling process, we utilize both an unsupervised aggregation approach-- data programming-- and a supervised random forest to obtain our estimated labels and ground our weakly supervised signals on the humanly annotated TOP training data. 

% Note that we train all approaches phase-wise. That is, we first select all trials according to Phase 1, train the labeling model, and predict outcome labels for all Phase 1 trials, before moving on to Phase 2. For data programming, we add TOP training labels to all of our other weakly supervised LFs. We duplicate TOP labels 3 times to obtain high agreement and therefore high weight in the matrix completion step.
% For our supervised approach, we train a Random Forest model on all other weakly supervised LF outputs to predict the ground truth. 

% % \newpage
% % \section*{CTO Statistics}
% % \subsection*{Labeling Function Statistics}
% % Table~\ref{tab:all_lf_stats} and Table~\ref{tab:all_lf_stats2} show statistics of all tunable and static labeling functions for the TOP training and validation data splits. We see that most LFs cover more than 50\% of the data, although this is not true of news headlines and status. Additionally, each individual accuracy scores and kappa values are generally not stellar on their own, with the highest kappa being status (which suffers from low coverage). In terms of kappa values, p-values from the tunable LFs and GPT decisions stand out from the static LFs as the highest, which makes sense as studies with more significant results may be one of the original annotator's primary signals and would also be referred to in the publications. The highest accuracy is status and GPT. Since status predicts all negative, it is clear that terminated, withdrawn, and incomplete trials in general are considered unsuccessful.

% % \begin{table}[ht]
% % \centering
% % \caption{Table of all \textit{static (i.e. not thresholded)} statistics of the different labeling functions that we consider for \method. Pos. Prop. refers to the positive percentage of all valid labels (i.e. $\frac{\#1}{\#1+\#0}$). Coverage indicates the proportion of TOP trials for that phase that the LF has predictions on. Acc. indicates raw accuracy compared to TOP train and valid split, and $\kappa$ denotes cohen kappa as well.}

% % \label{tab:all_lf_stats2}
% % \resizebox{.95\linewidth}{!}{
% % \begin{tabular}{c|cccccccc}
% % Phase & Labeling Function & Abstain & Predict 0 & Predict 1 & Pos. Prop. & Coverage & Acc & $\kappa$ \\ \toprule
% % \multirow{5}{*}{1} & status & 814 & 347 & 0 & 0.000 & 0.217 & 0.954 & 0.000 \\
% %  & gpt & 179 & 41 & 198 & 0.828 & 0.150 & 0.890 & 0.678 \\
% %  & linkage & 0 & 496 & 573 & 0.536 & 0.670 & 0.516 & 0.035 \\
% %  & stock\_price & 0 & 95 & 130 & 0.578 & 0.141 & 0.540 & -0.021 \\
% %  & results\_reported & 0 & 800 & 361 & 0.311 & 0.727 & 0.455 & -0.059 \\ \midrule
% % \multirow{5}{*}{2} & status & 3296 & 1155 & 0 & 0.000 & 0.228 & 0.968 & 0.000 \\
% %  & gpt & 683 & 338 & 913 & 0.730 & 0.247 & 0.875 & 0.707 \\
% %  & linkage & 0 & 2125 & 2027 & 0.488 & 0.820 & 0.576 & 0.150 \\
% %  & stock\_price & 0 & 457 & 447 & 0.494 & 0.178 & 0.504 & 0.008 \\
% %  & results\_reported & 0 & 2058 & 2393 & 0.538 & 0.879 & 0.524 & 0.050 \\ \midrule
% % \multirow{5}{*}{3} & status & 2999 & 439 & 0 & 0.000 & 0.121 & 0.954 & 0.000 \\
% %  & gpt & 605 & 276 & 1389 & 0.834 & 0.460 & 0.908 & 0.717 \\
% %  & linkage & 0 & 1284 & 1929 & 0.600 & 0.888 & 0.626 & 0.209 \\
% %  & stock\_price & 0 & 438 & 528 & 0.547 & 0.267 & 0.550 & 0.057 \\
% %  & results\_reported & 0 & 1399 & 2039 & 0.593 & 0.951 & 0.619 & 0.199 \\ \bottomrule
% % \end{tabular}
% % }
% % \end{table}

% % \begin{table}[ht]
% % \centering
% % \caption{Table of all statistics of the different \textit{tunable (by varying the quantile threshold)} labeling functions that we consider for \method. Pos. Prop. refers to the positive percentage of all valid labels (i.e. $\frac{\#1}{\#1+\#0}$). Coverage indicates the proportion of TOP trials for that phase that the LF has predictions on. Acc. indicates raw accuracy compared to TOP train and valid split, and $\kappa$ denotes cohen kappa as well.}
% % \label{tab:all_lf_stats}
% % \resizebox{\linewidth}{!}{
% % % \Huge
% % \begin{tabular}{c|ccccccccc}
% % Phase & \begin{tabular}[c]{@{}c@{}}Labeling \\ Function\end{tabular} & \begin{tabular}[c]{@{}c@{}}Best \\ Quantile\end{tabular} & Abstain & 0 & 1 & \begin{tabular}[c]{@{}c@{}}Pos. \\ 
% % Prop.\end{tabular} & Coverage & Acc & $\kappa$ \\ \toprule
% % \multirow{12}{*}{I} & update\_more\_recent & 0.8 & 88 & 665 & 408 & 0.380 & 0.672 & 0.564 & 0.153 \\
% %  & sites & 0.1 & 0 & 588 & 491 & 0.455 & 0.676 & 0.543 & 0.092 \\
% %  & serious\_ae & 0.9 & 0 & 22 & 339 & 0.939 & 0.226 & 0.490 & -0.045 \\
% %  & pvalues & 0.5 & 0 & 33 & 23 & 0.411 & 0.035 & 0.585 & 0.256 \\
% %  & patient\_drop & 0.9 & 0 & 4 & 220 & 0.982 & 0.140 & 0.530 & 0.013 \\
% %  & num\_sponsors & 0.7 & 0 & 1064 & 97 & 0.084 & 0.727 & 0.446 & -0.017 \\
% %  & num\_patients & 0.2 & 0 & 126 & 235 & 0.651 & 0.226 & 0.723 & 0.441 \\
% %  & news\_headlines & 0.7 & 637 & 16 & 48 & 0.750 & 0.040 & 0.610 & 0.009 \\
% %  & death\_ae & 0.1 & 0 & 37 & 324 & 0.898 & 0.226 & 0.553 & 0.086 \\
% %  & amendments & 0.1 & 0 & 30 & 195 & 0.867 & 0.141 & 0.715 & -0.076 \\
% %  & all\_ae & 0.9 & 0 & 6 & 355 & 0.983 & 0.226 & 0.509 & -0.010 \\ \midrule
% % \multirow{12}{*}{II} & update\_more\_recent & 0.8 & 290 & 2897 & 1264 & 0.304 & 0.822 & 0.530 & 0.051 \\
% %  & sites & 0.9 & 0 & 2723 & 1398 & 0.339 & 0.814 & 0.537 & 0.059 \\
% %  & serious\_ae & 0.9 & 0 & 211 & 2179 & 0.912 & 0.472 & 0.488 & -0.031 \\
% %  & pvalues & 0.5 & 0 & 418 & 341 & 0.449 & 0.150 & 0.683 & 0.384 \\
% %  & patient\_drop & 0.9 & 0 & 100 & 1614 & 0.942 & 0.338 & 0.533 & 0.003 \\
% %  & num\_sponsors & 0.9 & 0 & 4328 & 123 & 0.028 & 0.879 & 0.515 & -0.007 \\
% %  & num\_patients & 0.3 & 0 & 869 & 1524 & 0.637 & 0.472 & 0.699 & 0.398 \\
% %  & news\_headlines & 0.9 & 2678 & 24 & 68 & 0.739 & 0.018 & 0.608 & -0.007 \\
% %  & death\_ae & 0.1 & 0 & 155 & 2235 & 0.935 & 0.472 & 0.515 & 0.023 \\
% %  & amendments & 0.1 & 0 & 57 & 847 & 0.937 & 0.178 & 0.633 & -0.026 \\
% %  & all\_ae & 0.9 & 0 & 146 & 2244 & 0.939 & 0.472 & 0.483 & -0.041 \\ \midrule
% % \multirow{12}{*}{III} & update\_more\_recent & 0.9 & 217 & 1431 & 1790 & 0.556 & 0.891 & 0.513 & -0.012 \\
% %  & sites & 0.8 & 0 & 1091 & 1902 & 0.635 & 0.827 & 0.527 & -0.017 \\
% %  & serious\_ae & 0.9 & 0 & 708 & 1322 & 0.651 & 0.561 & 0.597 & 0.060 \\
% %  & pvalues & 0.5 & 0 & 449 & 896 & 0.666 & 0.372 & 0.768 & 0.450 \\
% %  & patient\_drop & 0.9 & 0 & 587 & 1210 & 0.673 & 0.497 & 0.609 & 0.053 \\
% %  & num\_sponsors & 0.1 & 0 & 2505 & 933 & 0.271 & 0.951 & 0.367 & -0.124 \\
% %  & num\_patients & 0.2 & 0 & 80 & 1959 & 0.961 & 0.564 & 0.759 & 0.182 \\
% %  & news\_headlines & 0.9 & 2734 & 26 & 72 & 0.735 & 0.027 & 0.696 & 0.077 \\
% %  & death\_ae & 0.9 & 0 & 61 & 1969 & 0.970 & 0.561 & 0.720 & 0.029 \\
% %  & amendments & 0.1 & 0 & 55 & 911 & 0.943 & 0.267 & 0.717 & -0.001 \\
% %  & all\_ae & 0.9 & 0 & 876 & 1154 & 0.568 & 0.561 & 0.540 & 0.015 \\ \bottomrule
% % \end{tabular}
% % }
% % \end{table}

% % % \newpage
% % % \subsection*{Statistics on Trial Linkage}
% % % \begin{figure}[ht]
% % %     \centering
% % %     \includegraphics[width=\linewidth]{figures/Trial_linkage_statistics.pdf}
% % %     \caption{Overview of the weak labels extracted from the trial linkage.}
% % %     \label{fig:trial_linkage_feat_ablation}
% % % \end{figure}

% % % \newpage
% % % \subsection*{Statistics on LLM Predictions}
% % % \label{supplementary: Statistics on LLM Predictions}

% % % \begin{figure}[ht]
% % %     \centering
% % %     \includegraphics[width=\linewidth]{figures/LLM_predictions_figure.pdf}
% % %     \caption{Overview of the weak labels from LLM predictions on PubMed abstracts.}
% % %     \label{fig:LLM_predictions_statistics}
% % % \end{figure}
% % \clearpage
% % \subsection*{Statistics on Trial Linkage}
% % \begin{figure}[ht]
% %     \centering
% %     \includegraphics[width=\linewidth]{figures/Trial_linkage_statistics.pdf}
% %     \caption{Overview of the weak labels extracted from the trial linkage.}
% %     \label{fig:trial_linkage_stats}
% % \end{figure}

% % We present statistics on the weak trial outcome labels extracted from the clinical trial linkages in  Figure~\ref{fig:trial_linkage_stats}. Figure~\ref{fig:trial_linkage_stats} A shows the phase distribution of these weak labels, excluding trials with missing phase information or labeled as 'Not Applicable', as they are omitted from our linking algorithm. Additionally, outcomes for Phase 4 are not included because there are no subsequent trials for Phase 4. The criteria for extracting labels for trial linkage are defined as follows:
% % \begin{equation}
% %     \text{Trial outcome} = \begin{cases}
% % \text{Success} & \text{if next phase trial exists} \\
% % \text{Not Sure} & \text{if there is a weakly connected next phase trial} \\
% % \text{Failure} & \text{if no next phase trial found} 
% % \end{cases}
% % \end{equation}

% % Here, a "weakly connected next phase trial" refers to a trial link found during the retrieval stage that received a negative cross-encoder score during the predict linkage stage. Figure~\ref{fig:trial_linkage_stats} B and C illustrate the distribution of weak labels across different phases and over time (years).

% % % \newpage
% % % \clearpage
% % \subsection*{Statistics on LLM Predictions}
% % \label{supplementary: Statistics on LLM Predictions}

% % In Figure~\ref{fig:LLM_predictions_statistics}, we present the statistics of LLM predictions on PubMed abstracts, including a histogram showing the number of publications per trial. Figure~\ref{fig:LLM_predictions_statistics} A illustrates the phase distribution of the extracted weak labels, including rare phases such as terminated, recruiting, and completed. The LLM is prompted to predict the trial outcome based on the provided abstracts as 'Success', 'Failure', or 'Not Sure'. The distribution of weak labels over time (years) and across phases is shown in Figure~\ref{fig:LLM_predictions_statistics} B and C, respectively. The number of 'Failure' labels is relatively low compared to others, as trials with multiple publications are more likely to be successful. Additionally, Figure~\ref{fig:LLM_predictions_statistics} D presents the histogram for background, derived, and result-type publications for the trials.

% % \begin{figure}[ht]
% %     \centering
% %     \includegraphics[width=\linewidth]{figures/LLM_predictions_figure.pdf}
% %     \caption{Overview of the weak labels from LLM predictions on PubMed abstracts.}
% %     \label{fig:LLM_predictions_statistics}
% % \end{figure}
% % \newpage

% % % \subsection*{Statistics of \method\ dataset}
% % % % \mycomment{
% % % % \begin{figure}[ht]
% % % %     \centering
% % % %     \begin{subfigure}{0.49\linewidth}
% % % %         \centering
% % % %         \includegraphics[width=\linewidth]{figures/all_completion_before_2020_phase.pdf}
% % % %         \caption{All trials with completion dates before 2020\label{fig:overall_status_part1}}
% % % %         % \label{fig:a}
% % % %     \end{subfigure}
% % % %     \hfill
% % % %     \begin{subfigure}{0.49\linewidth}
% % % %         \centering
% % % %         \includegraphics[width=\linewidth]{figures/completion_dates_between_2020_to_2024_phase.pdf}
% % % %         \caption{Trials completed between 2020 and 2024}
% % % %         % \label{fig:b}
% % % %     \end{subfigure}
% % % %     \caption{Statistics of all \method\ labels}

% % % % \end{figure}

% % % % \begin{figure}[ht]
% % % %     \centering
% % % %     \begin{subfigure}{0.49\linewidth}
% % % %         \centering
% % % %         \includegraphics[width=\linewidth]{figures/pre_pie_chart_phase.pdf}
% % % %         \caption{Pre-2020 Split(small molecules only)}
% % % %         % \label{fig:c}
% % % %     \end{subfigure}
% % % %     \hfill
% % % %     \begin{subfigure}{0.49\linewidth}
% % % %         \centering
% % % %         \includegraphics[width=\linewidth]{figures/post_pie_chart_phase.pdf}
% % % %         \caption{Post-2020 Split (small molecules only)}
% % % %         % \label{fig:another}
% % % %     \end{subfigure}
% % % %     \caption{Distributions of phases in different splits of \method\ dataset\label{fig:overall_status_part2}}
% % % % \end{figure}}


% % % The total number of clinical trials in our dataset is 479761. There are a total of 429796 clinical trials in our \method\ dataset after removing trials with no phase information. 
% % % % Figure \andy{what figure} show the proportions of phases in different splits of our dataset.  


% % % \begin{figure}[ht]
% % %     \centering
% % %     \includegraphics[width=\linewidth]{figures/Mismatch labels between TOP and CTOD.pdf}
% % %     \caption{Distribution of differences of the labels between the human-annotated TOP dataset and our \method\ dataset across phases and trial statuses. A good observation from these plots is that some of the terminated trials have been labeled as success in the TOP dataset, whereas ours have correctly identified them as failed trials.}
% % %     \label{fig:Mismatch labels between TOP and CTOD}
% % % \end{figure}


% % % \andy{we need to update these for pre and post as well, also we need to change to pdf}

% % % commented out due to updating labels
% % % \begin{figure}[ht]
% % %     \centering
% % %     \includegraphics[width=0.8\linewidth]{figures/normalized_stacked_bar_plot.png}
% % %     \caption{Proportions of labels (failure: 0, success: 1) in each type of overall\_status in \method\ dataset}
% % %     \label{fig:normalized_stacked_bar}
% % % \end{figure}

% % %\begin{figure}[ht]
% %    % \centering
% %    % \includegraphics[width=.9\linewidth]{figures/combined_pie_charts_with_legend.png}
% %    % \caption{Proportions of Overall Status and Phases in the \method\ dataset}
% %    % \label{fig:overall_status_pie_chart}
% % %\end{figure}

% % % \newpage
% % % \subsection*{Trial Linkage in Detail}
% % % \label{app:Trial_Linkage_Continued}
% % % \textbf{1. Search space selection:} We begin by filtering the trials from connected phases based on their completion dates relative to the start date of $x$, ensuring that any linkage candidate must have concluded before the commencement of $x$. Furthermore, we refine the search space by filtering for trials with similar intervention characteristics as $x$, such as 'Drug', 'Biological', 'Device', etc. This step increases the likelihood of identifying relevant and meaningful connections.
    
% % % \textbf{2. Retrieve top-K:} From the filtered search space $\mathbf{Z}$, we retrieve top-K most similar past trials to $x$. We extract key features and encode them into dense embedding to represent both $x$ and trials in the search space ($z_i \in Z$) as follows: $x = \{x_{\text{I}},x_{\text{C}},x_{\text{T}},x_{\text{S}},x_{\text{E}}\}$,  $z_i =  \{z^i_{\text{I}},z^i_{\text{C}},z^i_{\text{T}},z^i_{\text{S}},z^i_{\text{E}}\}$.

% % % Where the subscript $I$ denotes intervention or drug, $C$ denotes condition or targeted disease, $T$ denotes official trial title, $S$ denotes trial summary, and $E$ denotes eligibility criteria.  
    
% % % We excluded the lead sponsor as a feature to represent the trial for this task due to two reasons: 1) During progress from phases, the sponsorship often changes depending on their funding capacity, and 2) Based on our ablation given in supplementary~\ref{supplementary: Ablation on Features for Trial Linkage}, the inclusion of lead sponsor adversely impacted agreement between extracted weak labels and the TOP dataset. We utilized PubMedBERT \cite{gu2021domain} from HuggingFace to obtain dense embeddings for each feature. This model, previously named PubMedBERT, was pre-trained on PubMed abstracts and PubMedCentral full-texts. For lengthy features like `brief summary' and `eligibility criteria', we chunked them into 512-token segments, encoded them, and obtained the final embedding by mean pooling. Utilizing these embeddings, we performed a semantic search to obtain top-K ($K = 32$) similar trials using the cosine similarity score aggregated across features as follows:
% % % $\text{similarity}(x,z_i) = \sum_{i \in \mathbf{F}}\frac{x^i.z_j^i}{||x^i||||z_j^i||}
% % % $,
% % %     % \begin{equation}
% % %     %     \text{aggregated cos\_sim}(x,z_i) = \sum_{j \in \mathbf{F}}\frac{x^j.z_i^j}{||x^j||||z_i^j||}
% % %     % \end{equation}
% % % Where $\mathbf{F} =$ \{I,C,T,S,E\}. We convert the intervention name of drugs to their generic name based on the data from DrugBank\footnote{https://go.drugbank.com/} for standardization.

% % % \textbf{3. Predict linkage} Given the large search space of clinical trials, the initial retrieval may return irrelevant candidates. To mitigate this and predict the most probable previous phase candidate for $x$, we employ a re-ranking strategy using cross-encoders, which are pre-trained to predict the relevance of a retrieved passage given a query. We utilize a cross-encoder $g_{\theta}$ pre-trained on MS-MARCO \cite{nguyen2016ms}, a large information retrieval corpus based on user search queries from Bing. We provide feature pairs as input to the cross-encoder, obtaining and aggregating their scores across features before the final Sigmoid activation layer as follows: $\text{Cross-encoder score}(x,z_i) = \sum_{j \in \mathbf{F}}g_{\theta}(x^i,z^i_j)$.
% % %     % \begin{equation}
% % %     %     \text{Cross-encoder score}(x,z_i) = \sum_{j \in \mathbf{F}}g_{\theta}(x^j,z^j_i)
% % %     % \end{equation}
% % % Based on the cross-encoder scores, we predict the linkage by considering the trials with the highest positive cross-encoder scores as the most probable previous phase trials of $x$.

% % \subsection*{Pair-wise Agreement Between Labeling Functions}
% % To analyze the agreement between the labeling functions and the final aggregated labels, we calculated pairwise agreement scores using Cohen's Kappa in the TOP data splits. These scores are shown in Figure~\ref{fig: Pairwise R1} and \ref{fig: Pairwise RF2} for random forest and data programming label aggregation, respectively. Each cell in the heatmap represents the agreement score between a pair of labeling functions. It is important to note that each labeling function does not cover all trials with weak labels. Therefore, while calculating Cohen's Kappa, we only considered the trials common to both labeling functions. For instance, there are no common trials with weak labels from 'status' and 'amendments,' so the corresponding cell is left blank.

% % In the context of random forest label aggregation, LLM predictions on PubMed abstracts, p-values, trial linkage, number of sites, and number of patients showed higher agreement with the final aggregated labels. Similar patterns were observed with labels aggregated using data programming. Notably, LLM predictions had high agreement with p-values, likely because the LLM considered the p-values provided in the abstracts to predict trial outcomes. Additionally, there was good agreement between LLM predictions on PubMed abstracts and other factors such as trial linkage and number of patients. 

% % \begin{figure}[ht]
% %     \centering
% %     \includegraphics[width=.8\linewidth]{figures/RF_pairwise_agreement.png}
% %     \caption{Pairwise agreement with the labeling functions (RF)}
% %     \label{fig: Pairwise R1} 
    
% % \end{figure}

% % \begin{figure}[ht]
% %     \centering
% %     \includegraphics[width=.8\linewidth]{figures/DP_pairwise_agreement.png}
% %     \caption{Pairwise agreement with the labeling functions (DP)}
% %     \label{fig: Pairwise RF2} 
    
% % \end{figure}

% \clearpage
% \section*{Ablation on Features for Trial Linkage}
% \label{supplementary: Ablation on Features for Trial Linkage}
% This section focuses on the ablation study conducted on the trial features for the trial linking algorithm. Figure~\ref{fig:trial_linkage_feat_ablation2} presents the comparison results with TOP and the outcome labels from the trial linkage created using individual features. The features "intervention," "official title," "brief summary," and "eligibility criteria" consistently achieved better performance across all phases. In contrast, "lead sponsor" performed the worst, likely because trial sponsors often change based on funding capacity, even when a trial progresses to the next phase.

% Additionally, Table~\ref{tab:feat_comb_trial_linkage} shows the performance of various combinations of trial features across phases. Combining all trial features except "lead sponsor" yielded better performance across all phases. Including "lead sponsor" features reduced the accuracy of the extracted weak outcome labels. However, adding "lead sponsor" improved performance for Phase 1 trials, as it is rare for a trial to change sponsors between Phase 1 and Phase 2. 

% \begin{figure}[ht]
%     \centering
%     \includegraphics[width=.8\linewidth]{figures/F1_Comparison_Across_Features.png}
%     \caption{Ablation study on the use of different trial features to predict trial linkages and the agreement of their extracted weak labels with TOP human-annotated data labels using F1 scores.}
%     \label{fig:trial_linkage_feat_ablation2}
% \end{figure}

% \begin{table}[ht]
% \centering
% \caption{Results of the ablation study on the different combinations of trial features to predict trial linkages and the agreement of their extracted weak labels with TOP human-annotated data labels using F1 scores. \textcolor{red}{$\downarrow$} indicates that adding the feature decreased the performance. \textcolor{green}{$\uparrow$} indicates that adding the feature improved the performance.}
% \label{tab:feat_comb_trial_linkage}
% \vspace{0.1cm}
% \resizebox{\linewidth}{!}{
% \begin{tabular}{c|c|c}
% Phase & Feature combination & F1
%  \\ \midrule
% \multirow{5}{*}{Phase 1} & Official title + Intervention & 0.645 \\
% & Official title + Intervention + Brief Summary & 0.6426 \textcolor{red}{$\downarrow$}\\
% & Official title + Intervention + Brief Summary + Eligibility & 0.6447\textcolor{green}{$\uparrow$}\\
% & Official title + Intervention + Brief Summary + Eligibility + Condition & 0.6532 \textcolor{green}{$\uparrow$}\\
% & Official title + Intervention + Brief Summary + Eligibility + Condition + Lead Sponsor & \textbf{0.6658} \textcolor{green}{$\uparrow$}\\ \midrule

% \multirow{5}{*}{Phase 2} & Official title + Intervention & 0.6027\\
% & Official title + Intervention + Brief Summary & 0.6042 \textcolor{green}{$\uparrow$} \\
% & Official title + Intervention + Brief Summary + Eligibility & 0.608 \textcolor{green}{$\uparrow$}\\
% & Official title + Intervention + Brief Summary + Eligibility + Condition & \textbf{0.6196} \textcolor{green}{$\uparrow$}\\
% & Official title + Intervention + Brief Summary + Eligibility + Condition + Lead Sponsor & 0.6189\textcolor{red}{$\downarrow$}\\ \midrule

% \multirow{5}{*}{Phase 3} & Official title + Intervention & 0.7323 \\
% & Official title + Intervention + Brief Summary & 0.7319\textcolor{red}{$\downarrow$}\\
% & Official title + Intervention + Brief Summary + Eligibility & 0.7379\textcolor{green}{$\uparrow$}\\
% & Official title + Intervention + Brief Summary + Eligibility + Condition & \textbf{0.7498}\textcolor{green}{$\uparrow$} \\
% & Official title + Intervention + Brief Summary + Eligibility + Condition + Lead Sponsor & 0.7384 \textcolor{red}{$\downarrow$}\\ \midrule

% \multirow{5}{*}{All} & Official title + Intervention & 0.6686\\
% & Official title + Intervention + Brief Summary & 0.6687\textcolor{green}{$\uparrow$}\\
% & Official title + Intervention + Brief Summary + Eligibility & 0.6737\textcolor{green}{$\uparrow$}\\
% & Official title + Intervention + Brief Summary + Eligibility + Condition & \textbf{0.6842}\textcolor{green}{$\uparrow$} \\
% & Official title + Intervention + Brief Summary + Eligibility + Condition + Lead Sponsor & 0.6796\textcolor{red}{$\downarrow$}\\ 
% \bottomrule
% \end{tabular}
% }

% \end{table}

% \clearpage

% \section*{Prompts for LLM Predictions on PubMed Abstracts}
% \label{supplementary: Prompts for LLM Predictions}

% In this section, we describe the method used to obtain LLM predictions on PubMed abstracts, including the statistical test results and question-answer pairs. An example of such a prompt is shown in Figure~\ref{fig:LLM_prompts}. Additionally, we provide two examples of input abstracts given to the LLM and their resulting outputs, as shown in Figures~\ref{fig:GPT_response example} and \ref{fig:GPT_response example2}.

% \begin{figure}[t!]
%     \centering
%     \includegraphics[width=\linewidth]{figures/LLM_prompts.pdf}
%     \caption{LLM Prompts.}
%     \label{fig:LLM_prompts}
% \end{figure}

% \begin{figure}[ht]
%     \centering
%     \includegraphics[width=\linewidth]{figures/GPT_response_example_1.pdf}
%     \caption{Example response from GPT-3.5.}
%     \label{fig:GPT_response example}
% \end{figure}

% \begin{figure}[ht]
%     \centering
%     \includegraphics[width=\linewidth]{figures/GPT_response_example_2.pdf}
%     \caption{Example response 2 from GPT-3.5.}
%     \label{fig:GPT_response example2}
% \end{figure}
% \clearpage
% \newpage
% \newpage

% \section*{Case studies}
% We utilized our random forest labels for the following case studies.

% \subsection*{Case study 1} We conducted a case study on clinical trial NCT01213160\footnote{\url{https://clinicaltrials.gov/study/NCT01213160}}. This trial was completed in 2013. Five different weak labels (GPT decision, trial linkage, stock price, sites, and amendment) suggest that the trial was successful. The link to the PubMed article for this trial is \url{https://ncbi.nlm.nih.gov/pmc/articles/PMC5502072/}, which also suggests that \textit{"AZD4547 was well tolerated in Japanese patients, with the best response of stable disease $\geq$ 4 weeks."} Therefore, we believe NCT01213160 was successful, as our CTO label suggests. We believe the TOP label for this trial is incorrect.

% \subsection*{Case study 2} Another clinical trial we examined in detail is NCT01111188\footnote{\url{https://clinicaltrials.gov/study/NCT01111188}}. This trial was terminated. Therefore, our label for this trial is Failure (label: 0). However, its TOP label is Success (label: 1), which is unlikely as the trial was not completed. Additionally, the GPT decision for the trial was 0, which means it thinks the PubMed abstract we collected suggests that the trial failed. \textit{"...all patients required dose delays during cycle 2 due to cytopenias, and the study team decided to stop the trial...with the primary toxicity being myelosuppression"}.


% \section*{Datasheet (Inspired from Good Practices in AI)}
% \paragraph{A.1\;\;\;\;Motivation}
% \begin{itemize}
%     \item \textbf{For what purpose was the dataset created?}
    
%     We created \method\ to democratize clinical trial outcome prediction, which was previously only available to industry-sponsored researchers. Furthermore, we attempt to expand the previous labeling efforts (which were primarily focused on small drug interventions) and predict labels on all trials.
    
%     \item \textbf{Who created the dataset (e.g., which team, research group) and on behalf of which entity (e.g., company, institution, organization)?}
    
%     The authors of this paper.

%     \item \textbf{Who funded the creation of the dataset? If there is an associated grant, please provide the name of the grantor and the grant name and number.}

%     This work was supported by NSF award SCH-2205289, SCH-2014438, and IIS-2034479.
    
% \end{itemize}

% \paragraph{A.2\;\;\;\;Composition}
% \begin{itemize}
%     \item \textbf{What do the instances that comprise the dataset represent (e.g., documents, photos, people, countries)?}
    
%     \method\ contains molecule SMILES strings, eligibility criteria, ICD Codes, drug names, diseases, study status, phase information, and our automatically created labels. Furthermore, we also have additional QA tasks as extracted by GPT 3.5 Turbo 0125, news articles mined for the top 1000 industry sponsors, and stock prices.

%     \item \textbf{How many instances are there in total (of each type, if appropriate)?}

%     There is a total of 479,761 trials, each with multiple types of predicted labels via random forest and data programming, as well as each phase-optimized threshold. For small-molecule drug interventions, we also have SMILES and ICD Codes. 
%     We release all such labels to not limit any downstream use. Furthermore, there are a total of 1,115,017 news articles we extracted and 105,570 trials with corresponding QA pairs.
    
%     \item \textbf{Does the dataset contain all possible instances or is it a sample (not necessarily random) of instances from a larger set?}

%     % We will provide all instances in our GitHub repository for EHRXQA\footnote{\href{https://github.com/baeseongsu/ehrxqa}{\texttt{https://github.com/baeseongsu/ehrxqa}}} and MIMIC-CXR-VQA\footnote{\href{https://github.com/baeseongsu/mimic-cxr-vqa}{\texttt{https://github.com/baeseongsu/mimic-cxr-vqa}}}.
%     We provide all possible trial labels up to the beginning of May 2024. 

%     \item \textbf{What data does each instance consist of?}

%     \method\ contains molecule eligibility criteria, drug names, diseases, study status, phase information, and our automatically created labels. 
    
%     \item \textbf{Is there a label or target associated with each instance?}

%     The automatically predicted label is provided for each question.

%     \item \textbf{Is any information missing from individual instances? If so, please provide a description, explaining why this information is missing (e.g., because it was unavailable). This does not include intentionally removed information, but might include, e.g., redacted text.}
    
%     No.

%     \item \textbf{Are relationships between individual instances made explicit (e.g., users' movie ratings, social network links)?}

%     No.

%     \item \textbf{Are there recommended data splits (e.g., training, development/validation, testing)?}

%     Yes, please see Table \ref{tab:humanlabel} for a split of training trials with completion date $<2022$ tested on trials with completion date $\geq 2022$. 

%     \item \textbf{Are there any errors, sources of noise, or redundancies in the dataset?}

%     Automatically created labels inherently come with an element of noise. However, our high agreement with TOP's human labels (up to 0.91 F1), implies that our labels are of high quality.

%     % Questions are created by filling the slots in the templates with pre-defined values and records from the database. Thus, some questions can be grammatically incorrect but not critical (e.g, verb tense).

%     \item \textbf{Is the dataset self-contained, or does it link to or otherwise rely on external resources (e.g., websites, tweets, other datasets)?}

%     \method\ depends on multiple open source datasets.
%     \begin{enumerate}
%         \item CTTI: \url{https://ctti-clinicaltrials.org/} 
%         \item DrugBank \url{https://drugbank.com/}
%         \item PubMed \url{https://pubmed.ncbi.nlm.nih.gov/}
%     \end{enumerate}

    
%     % EHRXQA depends on three open-source databases: MIMIC-IV\footnote{\url{https://physionet.org/content/mimiciv/2.2/}}, MIMIC-CXR\footnote{\url{https://physionet.org/content/mimic-cxr/2.0.0/}}, and Chest ImaGenome\footnote{\url{https://physionet.org/content/chest-imagenome/1.0.0/}}, which are accessible via PhysioNet\footnote{\url{https://physionet.org/}}. 
%     % MIMIC-CXR-VQA depends on two open-source databases: MIMIC-CXR and Chest ImaGenome.


%     \item \textbf{Does the dataset contain data that might be considered confidential (e.g., data that is protected by legal privilege or by doctor-patient confidentiality, data that includes the content of individuals' non-public communications)?}

%     No. We obtained all data sources via open-source methods.

%     \item \textbf{Does the dataset contain data that, if viewed directly, might be offensive, insulting, threatening, or might otherwise cause anxiety?}

%     No.

%     \item \textbf{Does the dataset relate to people?}

%     Yes.

%     \item \textbf{Does the dataset identify any subpopulations (e.g., by age, gender)?}
    
%     Yes, but only in the eligibility criteria of the trials, which are public.

%     \item \textbf{Does the dataset contain data that might be considered sensitive in any way (e.g., data that reveals race or ethnic origins, sexual orientations, religious beliefs, political opinions or union memberships, or locations; financial or health data; biometric or genetic data; forms of government identification, such as social security numbers; criminal history)?}

%     No. There is no reference to individuals.
    
% \end{itemize}


% \paragraph{A.3\;\;\;\;Collection process}
% \begin{itemize}
%     \item \textbf{How was the data associated with each instance acquired?}

%     We automatically mined each LLM prediction, trial linkage, news headline, and stock price as an overview in Section \method\ Overview.

%     \item \textbf{What mechanisms or procedures were used to collect the data (e.g., hardware apparatuses or sensors, manual human curation, software programs, software APIs)?}
    
%     We mainly used Google Sheets and Python to collect, process, and label the data.
%     In addition, we used OpenAI's ChatGPT (GPT-3.5-turbo 0125) to generate QA and GPT outcome predictions.

%     \item \textbf{If the dataset is a sample from a larger set, what was the sampling strategy (e.g., deterministic, probabilistic with specific sampling probabilities)?}

%     Some data splitting was done according to previous data splits from TOP \url{https://github.com/futianfan/clinical-trial-outcome-prediction}. Additionally, we also split the data according to the following dates: $(-\infty,2018, 2020, \infty)$
        
%     \item \textbf{Who was involved in the data collection process (e.g., students, crowd workers, contractors) and how were they compensated (e.g., how much were crowd workers paid)?}

%     The authors of the paper collected and processed the data.

%     \item \textbf{Over what timeframe was the data collected?}

%     We collected the data between December 2023 and April 2024.

%     \item \textbf{Were any ethical review processes conducted (e.g., by an institutional review board)?}

%     N/A.

%     \item \textbf{Does the dataset relate to people?}

%     Yes.

%     \item \textbf{Did you collect the data from the individuals in question directly, or obtain it via third parties or other sources (e.g., websites)?}

%     N/A.

%     \item \textbf{Were the individuals in question notified about the data collection?}

%     N/A.

%     \item \textbf{Did the individuals in question consent to the collection and use of their data?}

%     N/A.

%     \item \textbf{If consent was obtained, were the consenting individuals provided with a mechanism to revoke their consent in the future or for certain uses?}

%     N/A.

%     \item \textbf{Has an analysis of the potential impact of the dataset and its use on data subjects (e.g., a data protection impact analysis) been conducted?}

%     The dataset does not have individual-specific information.
% \end{itemize}


% \paragraph{A.4\;\;\;\;Preprocessing/cleaning/labeling}
% \begin{itemize}
%     \item \textbf{Was any preprocessing/cleaning/labeling of the data done (e.g., discretization or bucketing, tokenization, part-of-speech tagging, SIFT feature extraction, removal of instances, processing of missing values)?}

%     N/A.

%     \item \textbf{Was the ``raw'' data saved in addition to the preprocess/cleaned/labeled data (e.g., to support unanticipated future uses)?}

%     N/A.

%     \item \textbf{Is the software that was used to preprocess/clean/label the data available?}

%     Preprocessing, cleaning, and labeling are done via Google Sheets and Python.   
% \end{itemize}

% \paragraph{A.5\;\;\;\;Uses}
% \begin{itemize}
%     \item \textbf{Has the dataset been used for any tasks already?}

%     No.

%     \item \textbf{Is there a repository that links to any or all papers or systems that use the dataset?}

%     No.

%     \item \textbf{What (other) tasks could the dataset be used for?}

%     Our dataset is designed to promote research primarily in clinical trial outcome prediction. The dataset can also be used for stock price/trend prediction, question answering, etc. 

%     \item \textbf{Is there anything about the composition of the dataset or the way it was collected and preprocessed/cleaned/labeled that might impact future uses?}

%     N/A.

%     \item \textbf{Are there tasks for which the dataset should not be used?}

%     N/A.
% \end{itemize}


% \paragraph{A.6\;\;\;\;Distribution}
% \begin{itemize}
%     \item \textbf{Will the dataset be distributed to third parties outside of the entity (e.g., company, institution, organization) on behalf of which the dataset was created?}

%     No.

%     \item \textbf{How will the dataset be distributed?}

%     Since clinical trial data is frequently updated, we provide the code for generating our CTO dataset at \url{https://github.com/chufangao/CTOD}. The current version of the dataset can be accessed at \url{https://zenodo.org/doi/10.5281/zenodo.11535960}.
    
%     % The datasets will be released at \href{https://github.com/baeseongsu/ehrxqa}{\texttt{https://github.com/baeseongsu/ehrxqa}} and \href{https://github.com/baeseongsu/mimic-cxr-vqa}{\texttt{https://github.com/baeseongsu/mimic-cxr-vqa}} upon publication.

%     \item \textbf{Will the dataset be distributed under a copyright or other intellectual property (IP) license, and/or under applicable terms of use (ToU)?}

%     The dataset is released under MIT License.

%     \item \textbf{Have any third parties imposed IP-based or other restrictions on the data associated with the instances?}

%     No.

%     \item \textbf{Do any export controls or other regulatory restrictions apply to the dataset or to individual instances?}

%     No.
% \end{itemize}


% \paragraph{A.7\;\;\;\;Maintenance}
% \begin{itemize}
%     \item \textbf{Who will be supporting/hosting/maintaining the dataset?}

%     The authors of this paper.

%     \item \textbf{How can the owner/curator/manager of the dataset be contacted(e.g., email address)?}
    
%     Contact the corresponding authors (\texttt{chufan2@illinois.edu} \& \texttt{jp65@illinois.edu} \& \texttt{trishad2@illinois.edu} \& \texttt{jimeng@illinois.edu}).

%     \item \textbf{Is there an erratum?}

%     No.

%     \item \textbf{Will the dataset be updated (e.g., to correct labeling errors, add new instances, delete instances)?}

%     If any corrections are needed, we plan to upload an updated version of the dataset along with detailed explanations of the changes. 

%     \item \textbf{If the dataset relates to people, are there applicable limits on the retention of the data associated with the instances (e.g., were the individuals in question told that their data would be retained for a fixed period of time and then deleted)?}

%     N/A

%     \item \textbf{Will older versions of the dataset continue to be supported/hosted/maintained?}

%     Primarily, we aim to keep only the latest version of the dataset. However, in specific cases like major updates to the dataset or the necessity to validate previous research with older versions, we will exceptionally retain past versions of the dataset for up to one year.

%     \item \textbf{If others want to extend/augment/build on/contribute to the dataset, is there a mechanism for them to do so?}

%     Contact the authors of this paper or raise a github issue.
% \end{itemize}
% % \section*{User Manual: Instructions to Generate and Use CTO}
% % We provide documentation to use CTO as of June 2024, and we will attempt to update this document over time as our sources update. However, the most up-to-date information can be seen in our GitHub \url{https://github.com/chufangao/CTOD}. The current version of the dataset can be accessed at \url{https://zenodo.org/doi/10.5281/zenodo.11535960}.

% % \subsection*{Instructions to Generate Clinical Trial Linkage}
% % The code to reproduce clinical trial linkages in the CTO dataset from the CTTI dataset is provided in the GitHub repository under the \texttt{/clinical\_trial\_linkage} folder. The step-by-step instructions to generate the clinical trials linkages are as follows:

% % \paragraph{Prerequisites:}
% % \begin{itemize}
% %     \item Download the \url{https://fda.gov/media/76860/download?attachment}{FDA orange book} and save it to ./FDA\_approvals/.  Currently, we provide the downloaded version as of 2024-04, which was used to create our dataset. Refer to \url{https://fda.gov/drugs/drug-approvals-and-databases/orange-book-data-files} for additional details on the FDA orange book.
% %     \item Download the trial dataset from CTTI <path>. If it has already been downloaded, provide the path to the data in the scripts.
% %     \item Download the National Drug Code Directory /drug/ndc: \url{https://open.fda.gov/data/downloads/}
% %     \item Download the DrugBank full database for researchers: 
    
% %     e.g. \url{https://go.drugbank.com/releases/latest}

% % \end{itemize}

% % \paragraph{1. Extract trial info and save trial embeddings:} First, we extract trial features from the CTTI dataset. Provide the <data\_path> for downloaded CTTI data in the command below:
% % \begin{verbatim}
% % cd clinical_trial_linkage
% % python extract_trial_info.py --data_path <CTTI dir>
% % \end{verbatim}
% % Run the following command to extract and save the embeddings for the trial features using PubMedBERT. Make sure to provide the path to save the embeddings. Feel free to make changes to num\_workers and gpu\_ids as necessary.
% % \begin{verbatim}
% % python get_embedding_for_trial_linkage.py 
% %     --root_folder <saved embeddings dir> 
% %     --num_workers 2 --gpu_ids 0,1
% % \end{verbatim}

% % \paragraph{2. Linking of clinical trials across phases:} Based on the extracted embeddings, we link the trials across different phases, as shown in the above figure. Run the following command to link the trials across phases. Provide the root\_folder path to save the extracted linkages and embedding\_path with the saved embeddings. Since we link from the latter phase to the initial phases, provide the starting later phase to target\_phase. Also, we need only to consider the following phases to create the trial linkage: \texttt{['Phase 2', 'Phase 2/Phase 3', 'Phase 3', 'Phase 4']}

% % \begin{verbatim}
% % # Phase 4
% % python create_trial_linkage.py --root_folder <created linkages dir>
% %     --target_phase 'Phase 4' --embedding_path <saved embeddings dir>
% %     --num_workers 2 --gpu_ids 0

% % # Phase 3
% % python create_trial_linkage.py --root_folder <created linkages dir>
% %     --target_phase 'Phase 3' --embedding_path <saved embeddings dir>
% %     --num_workers 2 --gpu_ids 0

% % # Phase 2/Phase 3
% % python create_trial_linkage.py --root_folder <created linkages dir>
% %     --target_phase 'Phase 2/Phase 3' --embedding_path <saved embeddings dir>
% %     --num_workers 2 --gpu_ids 0

% % # Phase 2
% % python create_trial_linkage.py --root_folder <created linkages dir>
% %     --target_phase 'Phase 2' --embedding_path <saved embeddings dir> 
% %     --num_workers 2 --gpu_ids 0
% % \end{verbatim}

% % \paragraph{3. Extract outcome labels:} Run the following command to extract clinical trial outcome weak labels from clinical trial linkages. Provide the path with saved trial linkages.
% % \begin{verbatim}
% % python extract_outcome_from_trial_linkage.py 
% %     --trial_linkage_path <trial linkage dir>
% % \end{verbatim}

% % \paragraph{4.  FDA approval matching:} Run the following command to match the FDA approvals from the orange book to phase 3 trials and update the outcome labels for phase 3 trials.
% % \begin{verbatim}
% % python match_fda_approvals.py --trial_linkage_path <matched trials path> 
% % \end{verbatim}

% % The final outcome labels extracted from the clinical trial linkages and matching FDA approvals will be saved at:
% % \begin{verbatim}
% % <trial linkage dir>/outcome_labels/Merged_(ALL)_trial_linkage_outcome_df.csv
% % \end{verbatim}

% % \subsection*{Instructions to Obtain LLM Predictions on PubMed Abstracts}
% % The code to obtain LLM predictions on the PubMed abstracts as of in the CTO dataset from the CTTI dataset is provided in the GitHub repository under the \texttt{/llm\_prediction\_on\_pubmed}
% %  folder. The step-by-step instructions are as follows:

% % \paragraph{Prerequisites:}
% % \begin{itemize}
% %     \item Download the trial dataset from CTTI. If it has already been downloaded, provide the path to the data in the scripts.
% %     \item To extract all the PubMed abstracts linked to the clinical trials, we use the NCBI API. Follow the instructions on this \url{https://support.nlm.nih.gov/knowledgebase/article/KA-05317/en-us} to create an NCBI account and obtain the API key.
% % \end{itemize}

% % \paragraph{1. Extract PubMed Abstracts:} Run the following commands for the extraction algorithm to retrieve all linked PubMed abstracts. Provide the NCBI API key, the path to the CTTI data, and the path to save the extracted abstracts.
% % \begin{verbatim}
% % cd llm_prediction_on_pubmed
% % python extract_pubmed_abstracts.py --data_path <CTTI dir> 
% %     --NCBI_api_key <API key> --save_path <Path to save extracted abstracts>
% % \end{verbatim}

% % \paragraph{2. Retrieve the Top 2 Abstracts:} To make the process efficient, we initially retrieve the top 2 most relevant abstracts (as shown in the figure above) and save them in a data frame.
% % \begin{verbatim}
% % python retrieve_top2_abstracts.py --data_path <Path to CTTI data> 
% %     --pubmed_path <extracted pubmed dir>
% % \end{verbatim}
% % The resultant data frame will be saved at \texttt{<pubmed\_path>/top\_2\_extracted\_pubmed\_articles.csv}

% % \paragraph{3. Get LLM Predictions:} To get the LLM prediction on PubMed abstracts, provide the OpenAI API key to the \texttt{get\_llm\_predictions.py} script and run the following. Also, provide the path to the above \texttt{top\_2\_extracted\_pubmed\_articles.csv} and the path to save LLM predictions. Along with the LLM predictions, extracted statistical features from the abstracts and the QA pairs are saved in the JSON files.

% % \begin{verbatim}
% % python get_llm_predictions.py 
% %     --top_2_pubmed_path <top_2_extracted_pubmed_articles.csv path> 
% %     --save_path <LLM predictions dir>
% % \end{verbatim}
% % Finally, run the following code to combine all the outcomes. Also, provide the path to the above \texttt{top\_2\_extracted\_pubmed\_articles.csv} and the path to saved LLM predictions.
% % \begin{verbatim}
% % python clean_and_extract_final_outcomes.py 
% %     --gpt_decisions_path <LLM predictions dir> 
% %     --top_2_pubmed_path <top_2_extracted_pubmed_articles.csv path>
% % \end{verbatim}

% % Final outcome predictions from LLM saved in \texttt{<top\_2\_pubmed\_path>/pubmed\_gpt\_outcomes.csv}

% % \subsection*{News Headlines}
% % \textbf{Prerequisites:}
% % \begin{itemize}
% % \item We use GNews to scrap Google News for the news headlines.
% % \end{itemize}

% % \textbf{1: Scrape Google News}
% % First, we extract trial features from the CTTI dataset. Provide the \texttt{<data\_path>} for downloaded CTTI data in the command below:

% % Run the following command to start the scraping for the top 1000 industry sponsors (NOTE: This will take a long time, i.e. on the scale of multiple weeks.) We share our scraped headlines in the Zenodo supplementary.

% % \begin{verbatim}
% % python get_news.py --mode=get_news
% % \end{verbatim}

% % \textbf{2: Obtaining Sentiment Embeddings from News Headlines and Study Titles}

% % Running this command also saves the news title embeddings and a dataframe of the news as \texttt{news.csv}.

% % \begin{verbatim}
% % python get_news.py --mode=process_news
% % \end{verbatim}

% % \textbf{3 Corresponding News and Trials:} We encode trial study title embeddings and obtain TopK Similarity. Running this command also saves study title embeddings.

% % \begin{verbatim}
% % python get_news.py --mode=correspond_news_and_studies 
% % \end{verbatim}


% % % \subsubsection{Labeling}
% % % \andy{complete}
% % % % \andy{add for news headlines and labeling}

% % \subsection*{Stock Price}
% % \textbf{Prerequisites:}

% % \begin{itemize}
% %     \item Download the trial dataset from CTTI. If it has already been downloaded, provide the path to the data in the scripts.
% %     \item Create a csv file `tickers.csv' that contains the names and corresponding tickers of sponsors in `name' and `ticker' columns respectively.
% %     \item Install yfinance from \url{https://pypi.org/project/yfinance/}
% % \end{itemize}

% % \textbf{1: Obtain Stock Prices:} Run \texttt{tickers\_2\_history.ipynb} to get historical stock prices for the sponsors in \texttt{tickers.csv} if those are available publicly. The stock price data will be stored in \texttt{stock\_prices\_historical.csv}.

% % \textbf{2: Calculate Slope:} Use \texttt{studies.txt} and \texttt{sponsors.txt} from CTTI with 
% % \texttt{stock\_prices\_historical.csv} and \texttt{tickers.csv} to calculate the slope of the stock prices using \texttt{slope\_calculation.ipynb}.


% % \subsection*{Running Baselines}
% % % \andy{trisha add baselines and stock price}
% % Here are the steps to run different baselines for clinical trial outcome prediction:

% % \paragraph{SPOT:} Update the train, test, and validation data paths in run\_spot.py. Execute the Python file:
% % \begin{verbatim}
% % python run_spot.py
% % \end{verbatim}

% % \paragraph{BioBERT:} Modify the train, test, and validation data paths in biobert\_trial\_outcome.py. Run the Python file:
% % \begin{verbatim}
% % python biobert_trial_outcome.py
% % \end{verbatim}

% % \paragraph{PubMedBERT:} Change the train, test, and validation data paths in pubmedbert\_trial\_outcome.py. Execute the Python file:
% % \begin{verbatim}
% % python pubmedbert_trial_outcome.py
% % \end{verbatim}

% % \paragraph{SVM, XGBoost, MLP, RF, or LR:} Ensure that the paths in baselines.py are correct. Run the Python file:
% % \begin{verbatim}
% % python baselines.py
% % \end{verbatim}


% \bibliography{custom}
% \bibliographystyle{unsrt}

% \end{document}
